# Supplementary material for: Analyzing the Evolution of Graphs and Texts
Source: arXiv:2411.06295 source file (2024-11-09)
Supplement: Supplementary file 1 [file appendix.tex]

\onecolumn
\section{Appendix}
\label{sec:appendix}
%\subsection{Changes in number}

\begin{table}[H]

    \centering
    \small
    \caption{Numerical difference between pre/post-edits in changed news titles: Most of them concern news dynamic updates of injuries and competition scores. High \textit{BERTScore} shows that numerical changes does not alter the meaning.}    
    \label{tab:numerical_changes}
    \tiny
   \begin{tabular}{p{0.03\textwidth}p{0.03\textwidth}p{0.3\textwidth}p{0.3\textwidth}p{0.05\textwidth}}
    \toprule
     Diff. &  Number & Before & After & BERTScore\\
     \midrule
      1.0 &     116  & louisiana floods lead to 6 deaths & louisiana floods lead to 7 deaths &        0.99 \\
      2.0 &      45 &yankees lead astros 1-0 in game 1: live score and updates & yankees lead astros 3-0 in game 1: live score and updates &       0.96 \\
      -1.0 &      31 &ransomware attack hits 23 texas towns, authorities say & ransomware attack hits 22 texas towns, authorities say &       0.99 \\
      3.0 &      24 &super bowl 2020 live: chiefs lead the 49ers, 7-3 & super bowl 2020 live: chiefs lead the 49ers, 10-3 &       0.93 \\
      4.0 &      17 &iraq: suicide bombing kills at least 18 in baghdad & iraq: suicide bombing kills at least 22 in baghdad &       0.98 \\
      5.0 &      14 & albania earthquake kills at least 8 & albania earthquake kills at least 13 &       0.97 \\
      100.0 &       6 & iran-iraq earthquake kills more than 300 & iran-iraq earthquake kills more than 400 &       0.98 \\
    \bottomrule
    \end{tabular}
\end{table}

\begin{table*}[htbp]
        \centering
        \caption{Breakdown of changed nouns. One pair may belong to more than one category}
        \label{tab:noun_changes}
        \tiny
    \hspace*{-0.00\textwidth}\begin{tabular}{ >{\raggedright\arraybackslash}p{0.1\textwidth} >{\raggedright\arraybackslash}p{0.03\textwidth} >{\raggedleft\arraybackslash}p{0.05\textwidth} >{\raggedright\arraybackslash}p{0.25\textwidth} >{\raggedright\arraybackslash}p{0.25\textwidth}}
    \toprule
     Category & Total & \%  & \makecell[l]{Examples (Before, After, \#)} & Description \\
    \midrule
     Share lemma & 132 & 15.33\% & \makecell[l]{(report, reports, 4); (riots, riot, 3)\\} & The change noun shares the lemma. \\
    \hline 
     Synonym & 65 & 7.54\% & \makecell[l]{(advisor, adviser, 3); (investigate, probe,2)\\} & The change noun is synonym. \\
    \hline 
     Minor & 109 & 12.65\% & \makecell[l]{(protestors, protesters, 5); (reelection, re-election,4)} & Only one character is changed (excluding same lemma pairs ) \\
    \hline 
     Hyponymn  & 33 & 3.83\% & \makecell[l]{(housing, home, 3); (semiconductor, chip, 2), \\(official, officer, 2); (supporter, believer, 1)} & Become more specific\\
    \hline 
     Hypernymn & 41 & 4.76\% & \makecell[l]{(snaps, photos, 5);(budget, plan, 2)} & Become more general  \\
     \hline 
     Others  & 481 & 55.86\% & \makecell[l]{(demo, democrats, 7); (4th, fourth, 4)\\(live, close, 4); (valuation, value, 3) } & All other noun changes \\
     \bottomrule
     All & 861 & 100\% & \makecell[l]{--} & All detected noun substitutions \\
     \bottomrule
    \end{tabular}
\end{table*}
    
\begin{table*}[htbp]
        \caption{Breakdown of changed verbs. One pair may belong to more than one category}
        \label{tab:verb_changes}

        \centering
        \tiny
    \hspace*{-0.00\textwidth}\begin{tabular}{ >{\raggedright\arraybackslash}p{0.1\textwidth} >{\raggedright\arraybackslash}p{0.03\textwidth} >{\raggedleft\arraybackslash}p{0.05\textwidth} >{\raggedright\arraybackslash}p{0.25\textwidth} >{\raggedright\arraybackslash}p{0.25\textwidth}}
    \toprule
     Category & Total & \%  & \makecell[l]{Examples (Before, After, \#)} & Description \\
    \midrule
     Share lemma & 135 & 23.56\% & \makecell[l]{(cancelled, canceled, 7); (shuts, shut, 2)\\} & The change noun shares the lemma. \\
    \hline 
     Synonym & 59 & 10.29\% & \makecell[l]{(rise, climb, 2); (blew, botched, 2)\\} & The change noun is synonym. \\
    \hline 
     Minor & 35 & 6.10\% & \makecell[l]{(eying, eyeing, 2); (targetting, targeting,2)} & Only one character is changed (excluding same lemma pairs ) \\
    \hline 
     Hyponymn  & 38 & 6.63\% & \makecell[l]{(drops, tumbles, 3); (pull, drag, 2)\\(mulls, considers, 2); (rejects, rebuffs, 2)} & Become more specific\\
    \hline 
     Hypernymn & 46 & 8.02\% & \makecell[l]{(passes, advances, 3);(linger, remain, 3)\\(breaking, damaging, 2); (reveals, shows, 1)} & Become more general  \\
     \hline 
     Others  & 260 & 45.37\% & \makecell[l]{(drop, slip, 3); (reveals, says, 3) } & All other noun changes \\
     \bottomrule
     All & 573 & 100\% & \makecell[l]{--} & All detected verb substitutions \\
     \bottomrule
    \end{tabular}
\end{table*}

\begin{table}[ht]
        \caption{\textit{Left}: The tracked news categories per agency. \textit{Right}: The headline modification ratio in each news category}
        \label{tab:in_changed_news_cate_ratio_agency}
    \scalebox{0.85}{
    \centering
    \tiny
    \begin{minipage}{0.55\textwidth}
    \begin{tabular}{lrrrrrr}
        \toprule
                 Domain &  Politics &  Business &  Entertainment &  Technology &  Top Stories &  Total \\
        \midrule
                    BBC &      1973 &      1562 &           1495 &         824 &            0 &   5854 \\
               BuzzFeed &       330 &        92 &           3928 &         195 &            0 &   4545 \\
                    CNN &      4548 &         1 &           1166 &         629 &            0 &   6344 \\
            Daily Beast &         0 &         0 &              0 &           0 &         4359 &   4359 \\
             Daily Mail &         0 &      3670 &          36312 &        1263 &        33873 &  75118 \\
               Fox News &      6307 &       108 &           4273 &         315 &            0 &  11003 \\
        Huffington Post &      2909 &        57 &           1902 &           7 &            0 &   4875 \\
            MarketWatch &         0 &         0 &              0 &           0 &         7503 &   7503 \\
        National Review &         0 &         0 &              0 &           0 &         3324 &   3324 \\
          New York Post &         0 &      1458 &           2018 &         514 &         9891 &  13881 \\
         New York Times &      2374 &      2983 &           3851 &         538 &            0 &   9746 \\
                Newsmax &       897 &        25 &            155 &          38 &            0 &   1115 \\
                    OAN &      2922 &      3545 &            528 &        1328 &            0 &   8323 \\
              The Blaze &         0 &         0 &              0 &           0 &         4401 &   4401 \\
        The Epoch Times &      3179 &      1077 &            193 &         316 &            0 &   4765 \\
           The Guardian &      3456 &       627 &           1874 &         959 &            0 &   6916 \\
               The Hill &         0 &         0 &              0 &           0 &         5676 &   5676 \\
        Washington Post &      2126 &      2014 &           1458 &         478 &            0 &   6076 \\
             Yahoo News &     11074 &    183653 &              7 &       32512 &            0 & 227246 \\
        \bottomrule
        \end{tabular}
    \end{minipage}%
    \begin{minipage}{0.55\textwidth}
        \begin{tabular}{lrrrrrr}
        \toprule
        Domain &  Politics &  Business &  Entertainment &  Technology &  Top Stories &  Total \\
        \midrule
        BBC             &    0.3082 &    0.2855 &         0.1371 &      0.0898 &       0.0000 & 0.2277 \\
        BuzzFeed        &    0.2576 &    0.0000 &         0.4812 &      0.2154 &       0.0000 & 0.4438 \\
        CNN             &    0.2419 &    0.0000 &         0.1612 &      0.0000 &       0.0000 & 0.2030 \\
        Daily Beast     &    0.0000 &    0.0000 &         0.0000 &      0.0000 &       0.1308 & 0.1308 \\
        Daily Mail      &    0.0000 &    0.0515 &         0.0592 &      0.0451 &       0.0970 & 0.0756 \\
        Fox News        &    0.0591 &    0.0926 &         0.0314 &      0.0571 &       0.0000 & 0.0486 \\
        Huffington Post &    0.0399 &    0.0877 &         0.0273 &      0.1429 &       0.0000 & 0.0357 \\
        MarketWatch     &    0.0000 &    0.0000 &         0.0000 &      0.0000 &       0.3453 & 0.3453 \\
        National Review &    0.0000 &    0.0000 &         0.0000 &      0.0000 &       0.0126 & 0.0126 \\
        New York Post   &    0.0000 &    0.0638 &         0.0852 &      0.0292 &       0.0650 & 0.0665 \\
        New York Times  &    0.2784 &    0.3144 &         0.0444 &      0.1375 &       0.0000 & 0.1892 \\
        Newsmax         &    0.0268 &    0.0400 &         0.0065 &      0.0000 &       0.0000 & 0.0233 \\
        OAN             &    0.0404 &    0.4886 &         0.0890 &      0.2108 &       0.0000 & 0.2616 \\
        The Blaze       &    0.0000 &    0.0000 &         0.0000 &      0.0000 &       0.0400 & 0.0400 \\
        The Epoch Times &    0.1787 &    0.0706 &         0.0259 &      0.1203 &       0.0000 & 0.1442 \\
        The Guardian    &    0.2922 &    0.3142 &         0.0326 &      0.1022 &       0.0000 & 0.1975 \\
        The Hill        &    0.0000 &    0.0000 &         0.0000 &      0.0000 &       0.0592 & 0.0592 \\
        Washington Post &    0.2413 &    0.1226 &         0.0501 &      0.1736 &       0.0000 & 0.1508 \\
        Yahoo News      &    0.2390 &    0.0713 &         0.0000 &      0.1073 &       0.0000 & 0.0846 \\
        \bottomrule
        \end{tabular}

    \end{minipage}
    }
\end{table}

\xingzhiswallow{

\begin{table}[H]
    \centering
    \caption{Examples of changed news headline with BERTScore}
    \label{tab:bert-score-example}

    \tiny
\begin{tabular}{>{\raggedright\arraybackslash}p{0.45\textwidth} >{\raggedright\arraybackslash}p{0.45\textwidth} >{\raggedleft\arraybackslash}p{0.05\textwidth} }
\toprule
                                                                    Before &                                                                                                                                                    After &  BERTScore\\
\midrule
                               Sir Jeffrey Donaldson and Micheál Martin to meet in Dublin &                                                                                                               Brexit: Irish support for deal harming NI, says DUP leader &         0.0260 \\
                             Pipeline officials hope most service will be back by weekend &                                                                                                             After Colonial pipeline attack, maneuvers to avert shortages &         0.0645 \\
                             Gold prices slip, head for steepest monthly slump since 2013 &                                                                                        Gold settles higher for session and quarter but logs month-end, first half losses &         0.1209 \\
            'I still don't believe Meghan': Piers Morgan tweets defiant Churchill message &                                                                                                Meghan Markle formally complained to ITV before Piers Morgan lost his job &         0.1802 \\
      Motorway speed limit is cut to 60mph to reduce illegally nitrogen dioxide emissions &                                                                          These are the stretches of road where you'll have to drive 10mph UNDER the national speed limit &         0.1813 \\
          Maya Jama is giddy as she teases her glam BRIT Awards look in her dressing room &                                                                                            BRIT Awards 2021: Maya Jama admits she's had no sleep ahead of hosting duties &         0.1979 \\
Stock market news live updates: Stock futures fall after Fed minutes highlight taper talk & Stock market news live updates: S\&P 500 ends slightly higher, rising for the first time in three sessions as investors eye earnings, better-than-expected jobless claims &         0.2261 \\
                               Dollar set for biggest rise in 7 days as virus cases climb &                                                                                                        U.S. dollar climbs as new virus outbreaks threaten global outlook &         0.2363 \\
                         Biden says he hopes the Chauvin jury reaches the “right verdict” &                                                          ‘At least, God, now there is some justice’: Biden says guilty verdict in Floyd murder offers a chance at reform &         0.2526 \\
  ‘That’s crazy!’ Take a look at the damage a lightning strike in Florida caused this car &                                                                                 Lightning hits Florida highway and sends a chunk of asphalt through a truck’s windshield &         0.2787 \\
                                           Covid and school: 'A little party never killed nobody' &                                                        Covid and school: Three ways US schools are responding &         0.3327 \\
                                   Asian markets fall for third day after shock US inflation rise &                                                      UK shares join global market sell-off on inflation fears &         0.3392 \\
                                   Stocks, European Futures Dip as Bond Yields Rise: Markets Wrap &                                               Yields Gain as Traders Absorb Biden Spending Plan: Markets Wrap &         0.3474 \\
                                     Dominic Raab under pressure from Tories and Labour to resign &                     Dominic Raab under pressure to quit after delegating ‘rescue call’ for Afghan translators &         0.3740 \\
Penn Badgley is spotted pushing a baby stroller while working on the upcoming third season of You &               You Season Three: Penn Badgley and Tati Gabrielle seen on set with baby stroller during filming &         0.3969 \\
                                  39 LGBTQ+ TV And Movie Characters Who Deserve Their Own Spinoff & 39 LGBTQ Characters We're So Obsessed With, We're Calling Hollywood And Demanding They Get Their Own Spinoffs &         0.3989 \\
                           As resettlement efforts advance, some Afghans face an uncertain future &                                           They made it out of Afghanistan. But their path ahead is uncertain. &         0.4185 \\
                                    Iran, world powers to hold nuclear talks in Vienna on Tuesday &                                            U.S, Iran to go to Vienna for indirect nuclear deal talks: sources &         0.4189 \\
                             Barclays to invest more than \$400 million to expand India operations &                               Barclays bets on India again with \$400 million infusion into investment banking &         0.4405 \\
                                   Gold prices attempt to halt 3-session skid ahead of Fed update &                                        Gold prices post first gain in 4 sessions, move lower after Fed update &         0.4855 \\
                                                      Puma reports strong sales despite port congestion, politics &                                                                          Puma sees sales hit from China backlash and freight delays &         0.5533 \\
                                                      Older Asian man robbed in SF laundromat ambush-style attack &                                                                   3 arrested in shocking attack on older Asian man in SF laundromat &         0.5701 \\
             Bob Odenkirk 'doing great' says co-star David Cross after the star collapsed on Better Call Saul set &                                         Bob Odenkirk, 58, 'doing great' and 'joking' again after collapsing on Better Call Saul set &         0.6476 \\
                                                 U.S. Sends Taiwan Shots; Brazil Deaths Top 500,000: Virus Update &                                                                     U.S. Sends Taiwan Shots; India Third Wave Warning: Virus Update &         0.6783 \\
When free doughnuts aren’t enough: It may take penalizing unvaccinated Americans to convince them to get the shot & When free doughnuts aren’t enough: Why monthly surcharges may be the way to convince unvaccinated Americans to get their COVID shot &         0.6815 \\
             Bethenny Frankel, 50, looks sensational during vacation with boyfriend Paul Bernon and daughter Bryn &                                    Bethenny Frankel wears swimsuit on Florida beach holiday with boyfriend Paul Bernon and daughter &         0.6975 \\
                                                  Australia Bids for Unemployment in 4s in Budget Spending Signal &                                                                         Australia Bids for Unemployment in 4s, Signals Fiscal Spend &         0.7388 \\
                                              Democrats Roll Out \$3.5 Trillion Budget to Fulfill Expansive Agenda &                                                             Democrats Roll Out \$3.5 Trillion Budget to Fulfill Biden’s Broad Agenda &         0.7796 \\
                                                Google to introduce measures to curb online financial scams in UK &                                                                           Google to clamp down on online financial scams in Britain &         0.7845 \\
                                                      U.S. Vaccine Patent Shock Roils Pharma as Talks Move to WTO &                                                                    U.S. Vaccine Patent Surprise Roils Pharma as WTO Debate Heats Up &         0.7962 \\
             Covid: Blips in the supply of vaccines will fall now 'bumps' are ironed out, pharma experts say &             Covid vaccine supply blips will fall now 'bumps' are ironed out, pharma experts say &         0.8085 \\
                          New Jersey to require masks in schools as Delta variant spreads, media reports say &                                 New Jersey to require masks in schools as Delta variant spreads &         0.8268 \\
Live updates Biden open to compromise on jobs and infrastructure but says ‘inaction simply is not an option’ & Biden open to compromise on jobs and infrastructure but says ‘inaction simply is not an option’ &         0.8530 \\
                    Nicola Sturgeon pictured with Muslim cleric who once compared gay marriage to bestiality &        Nicola Sturgeon seen in photo with Muslim cleric who compared gay marriage to bestiality &         0.8646 \\
                                                   US poised to impose sanctions on Russia for cyber-attacks &                                               US imposes sanctions on Russia over cyber-attacks &         0.8742 \\
                                            Homeowners to get 15 years to sue for bad workmanship - minister &                           Homeowners to get 15 years to sue for 'shoddy' workmanship - minister &         0.9016 \\
                                                    Apple v Epic: Tim Cook takes the stand in Epic legal row &                                  Apple v Epic: Tim Cook appeared on the stand in Epic legal row &         0.9239 \\
                               Gaetz and Greene Hold Bizarre Outdoors ‘Protest’ After Multiple Venues Bailed &                    Gaetz and Greene Hold Bizarre Outdoor ‘Protest’ After Multiple Venues Bailed &         0.9528 \\
                                                     Man surrenders after claiming to have bomb near Capitol &                                      Man surrenders after claiming to have bomb near US Capitol &         0.9529 \\
                            Using spyware against journalists ‘completely unacceptable’ – EU’s von der Leyen &                 Using spyware against journalists ‘completely unacceptable’ -EU’s von der Leyen &         0.9724 \\

\bottomrule
\end{tabular}
\end{table}

}

\begin{table}[H]
    \centering
    \tiny
    \caption{Examples of altered headlines. The \textit{first} part is the manually selected modifications. The \textit{second} part is sampled from our dataset by change category }
    \label{tab:category-example}
    \scalebox{0.85}{
\begin{tabular}{>{\raggedright\arraybackslash}p{0.43\textwidth} >{\raggedright\arraybackslash}p{0.43\textwidth} >{\raggedleft\arraybackslash}p{0.05\textwidth}>{\raggedleft\arraybackslash}p{0.08\textwidth}}
\toprule
                                                                                        Before &                                                                                                             After &  BERT-F1 &       Type \\
\midrule
One Dose of J.\&J. Vaccine Is Ineffective Against Delta, Study Suggests &	J.\&J. Vaccine May Be Less Effective Against Delta, Study Suggests & 0.6830 & other \\
Malawi burns thousands of Covid-19 vaccine doses&	Malawi burns thousands of expired AstraZeneca Covid-19 vaccine doses & 0.7217 & other \\
Biden to huddle with Senate Democrats on Covid relief ahead of push for passage&	Biden urges Senate Democrats to reject poison pills that could sink relief plan ahead of push for passage & 0.3777 & other \\
Australia to investigate two deaths for possible links to COVID-19 vaccine&	Australia says two deaths not likely to be linked to COVID-19 vaccine & 0.7236 & citation \\
Canada adds blood clot warning to AstraZeneca's COVID-19 vaccine &	Canada says AstraZeneca COVID-19 vaccine safe, but adds blood clot warning & 0.7546 & citation \\
China's Zhurong rover will land on Mars TONIGHT	& China's Zhurong rover will land on Mars 'in the next five days & 0.7234 & other \\
Nike chief executive says firm is 'of China and for China'	&Nike boss defends firm's business in China & 0.4559 & other \\
MAGA 2.0&	“A new bargain”: Biden’s 2024 tease bets big on nostalgia & 0.0257 & emotional \\
\midrule
                                                    At Least Eight People Died In A School Shooting In Russia &                                                                          At Least Nine People Died In A School Shooting In Russia &         0.9866 &  paraphrase \\
            India sees cases officially drop below 300,000 a day but now country threatened by killer cyclone &                                      India cases officially drop below 300,000 a day but now country threatened by killer cyclone &         0.9034 &  paraphrase \\
                                                %   90\% of all adults eligible for COVID-19 vaccine by April 19 &                                                                     90\% of all U.S. adults eligible for COVID vaccine by April 19 &         0.8448 &  paraphrase \\
                                            %   A 19th Century Theory Explains Why Consumers Might Not Splurge &                                                                      A 19th Century Theory Explains Why Consumers May Not Splurge &         0.9857 &  paraphrase \\
                                                %  The cost of living posts biggest surge since 2008, CPI shows &                                The cost of living posts biggest surge since 2008, CPI shows, as inflation spreads through economy &         0.8202 &  paraphrase \\
                                                        The Latest: UN: 38,000 Palestinians displaced in Gaza &                                                                         The Latest: Biden expresses 'support' for Gaza cease-fire &         0.4043 &  dyn update \\
                                    %   Dyson leak row: Don't lock ministers in ivory towers, says senior Tory &                                                                                  Starmer: PM can't distance himself from 'sleaze' &         0.2030 &  dyn update \\
                               August 5 at 2PM ET: Join Engine Media CEO and Executive Chairman Fireside Chat &                                                 August 5 at 2PM ET: Join Engine Media CEO and Executive Chairman in Fireside Chat &         0.9393 &  dyn update \\
                                            %  Plant-Based Food Use Rising ‘Unbelievably Fast’: Catalyst Update &                                                                    FTX Chief Sees Enduring Volatility for Crypto: Catalyst Update &         0.1229 &  dyn update \\
                                                %  Futures Steady Before Payrolls; Treasuries Dip: Markets Wrap &                                                                  Stocks, Treasury Yields Rise on Robust Jobs Report: Markets Wrap &         0.3799 &  dyn update \\
                                                                               23 Amazing Jokes From Hot Fuzz &                                                      23 Jokes From "Hot Fuzz" That Humans Will Laugh At For The Next 10,000 Years &         0.4715 & elaboration \\
                                % Dad’s Girlfriend Arrested After Child’s Body Found in Tote Bag at Texas Motel &                                   Dad of Boy Found Dead in Tote Bag at Texas Motel ‘Can Barely Breathe’ as Girlfriend Is Arrested &         0.5259 & elaboration \\
                                        %   Secrets of Prince William and Kate Middleton's big day 10 years ago &                                  Royal wedding secrets from Prince William and Kate Middleton's big day on their 10th anniversary &         0.5444 & elaboration \\
                                                 Official: Haiti President Jovenel Moïse assassinated at home &                                               Haiti President Jovenel Moïse assassinated at home; Biden calls it 'very worrisome' &         0.5179 & elaboration \\
                                %  'More explosions could occur': Thousands flee as volcano erupts in Caribbean &           'More explosions could occur': La Soufriere volcano eruption sends thousands fleeing on Caribbean island of St. Vincent &         0.6160 & elaboration \\
                                           Senator Capito says Republicans plan new U.S. infrastructure offer &                                                                          U.S. Senate Republicans prepare new infrastructure offer &         0.5434 &   concision \\
                                            % Caroline Jurie: Mrs World arrested over Sri Lanka pageant bust-up &                                                                                 Sri Lanka Mrs World arrested over pageant bust-up &         0.6387 &   concision \\
                            %   U.S. stock futures take retail sales, PPI data in stride as investors await Fed &                                                                 U.S. stocks edge lower after economic data as investors await Fed &         0.5774 &   concision \\
                      U.S. second-quarter economic growth revised slightly higher; weekly jobless claims rise &                                                                        U.S. second-quarter growth raised; corporate profits surge &         0.5540 &   concision \\
                                            % Right-Wing Media Attacks ‘Weak’ Simone Biles: ‘Selfish Sociopath’ &                                                                         Right-Wing Media Launches Unhinged Attack on Simone Biles &         0.4696 &   concision \\
                                                                                %   FKA twigs steps out in NYC &                                     FKA twigs steps out in NYC after claiming it was a 'relief' to speak out against Shia LaBeouf &         0.5539 &   emotional \\
                    %   Phoebe Dynevor Almost Quit Acting Before Her "Bridgerton" Audition With Regé-Jean Page &                                      Phoebe Dynevor Wanted To "Throw In The Towel" On Her Acting Career Right Before "Bridgerton" &         0.4885 &   emotional \\
                                                 Undercover police officers spied on Peter Hain over 25 years &                                                  Peter Hain accuses undercover police of lying over reports on apartheid campaign &         0.2465 &   emotional \\
% US surpasses 100M vaccinations; Pfizer vaccine appears effective against asymptomatic cases: COVID-19 updates &                        US surpasses 100M vaccinations; IRS begins sending first round of \$1,400 relief payments: COVID-19 updates &         0.4424 &   emotional \\
                                               Suspect arrested following series of Arizona traffic shootings &                                                     Arizona gunman goes on traffic shooting rampage, leaving one dead, 12 injured &         0.2247 &   emotional \\
                                            % 23 Funny "Brooklyn Nine-Nine" Memes To Get You Ready For Season 8 &                                                                                                Brooklyn Nine Nine Memes And Jokes &         0.2271 &  neutralize \\
                % Hundreds chanting 'Kill the Bill' protest in Bristol over controversial Police and Crime bill &                                    Protesters smash police windows and attack officers' van amid 'Kill the Bill' march in Bristol &         0.4220 &  neutralize \\
                %  Prince Philip will become 25th Royal in a 200-year-old vault hidden below St George's Chapel &                               Prince Philip to be buried in 200-year-old vault below St George's Chapel but only until Queen dies &         0.6037 &  neutralize \\
                                                 Raul Castro confirms he's resigning, ending long era in Cuba &                                                                        Raul Castro resigns as Communist chief, ending era in Cuba &         0.7310 &  neutralize \\
         Nikki Grahame's life will be celebrated in a new Channel 4 documentary four months on from her death &                                                                   Nikki Grahame to be commemorated in a new Channel 4 documentary &         0.6698 &  neutralize \\
                                        Fourth stimulus check update: Your next payment could be one of these &                                                                 Fourth stimulus check? These payments are already in the pipeline &         0.4479 & foward ref. \\
                                                                       12 Movie Opinions You Might Agree With &                                                     Here Are 12 More Movie Opinions I Strongly Believe, But Do You Agree With Me? &         0.4246 & foward ref. \\
                    % A park next to the White House that was closed amid protests last year partially reopens. &                                   Lafayette Park, which was closed amid protests at the White House last year, partially reopens. &         0.7430 & foward ref. \\
                                        %  Biden to share ‘next steps’ for COVID-19 booster program later today & People in the U.S. who were vaccinated with Moderna and Pfizer’s COVID-19 vaccines will be eligible for a third dose in September &         0.2475 & foward ref. \\
                                                %   ‘How I Got In’: A Harvard/Stanford/Wharton Admit Tells All &                                                                          How I Got In: A Harvard/Stanford/Wharton Admit Tells All &         0.7685 & foward ref. \\
                                                 Watch Jeff Bezos’ ‘Blue Origin’ launch into space live today &                                                Everything you need to know as Jeff Bezos’ ‘Blue Origin’ launches into space today &         0.6179 & personalize \\
                                The "Degrassi: TNG" Cast Is Reuniting In Honor Of The Show's 20th Anniversary &                                                      The "Degrassi" Cast Is Reuniting And I Am So Excited To Relive My Teen Years &         0.4838 & personalize \\
                        Stimulus Update: States Give Out Thousands of Bonus \$1,000 Checks To School Employees &                                             Stimulus Update: States Give Out Thousands of Bonus \$1,000 Checks – Will You Get One? &         0.7416 & personalize \\
        %  Chrissy Teigen shares embarrassing encounter with Michael Keaton while playing game on NBC talk show &                                   Chrissy Teigen reveals she once confused Hollywood legend Michael Keaton for a champagne WAITER &         0.3173 & personalize \\
    %   ‘Strong perception’ that Tory party is insensitive to Muslim communities, report finds – politics live &                       Boris Johnson says he would not repeat ‘offending language’ about Muslims as prime minister – politics live &         0.3395 & personalize \\
                                    Kendall Jenner Has Some Pretty Strong Thoughts About The Kardashian Curse &                                   Kendall Jenner Talked About The Kardashian Curse And Said "The Men Need To Take Responsibility" &         0.5229 &    citation \\
                                            %  Howard Beckett: Labour suspends union official after Patel tweet &                                                   Howard Beckett: Patel laws 'disgusting' says union boss after Labour suspension &         0.4986 &    citation \\
                  Afghan guard killed: Firefight leaves at least one dead and others injured at Kabul airport &                  'It would be better to die under Taliban rule than face airport crush', say US embassy's 'betrayed' Afghan staff &         0.0656 &    citation \\
                                                    %   Police: 3 officers stable after being shot in Delaware &                                                                       Police say threat over after 3 officers wounded in Delaware &         0.6105 &    citation \\
                                           Apple beats sales expectations on iPhone, services, China strength &                                                                    Apple says chip shortage reaches iPhone, growth forecast slows &         0.2611 &    citation \\
\bottomrule
\end{tabular}
}
\end{table}

\xingzhiswallow{
\begin{table}[H]
    \centering
    \tiny
    \caption{The examples of altered headlines. The first part is the manually selected modifications. The second part is sampled from our dataset by change category }
    \label{tab:category-example}

\begin{tabular}{>{\raggedright\arraybackslash}p{0.43\textwidth} >{\raggedright\arraybackslash}p{0.43\textwidth} >{\raggedleft\arraybackslash}p{0.05\textwidth}>{\raggedleft\arraybackslash}p{0.08\textwidth}}
\toprule
                                                                                        Before &                                                                                                             After &  BERT-F1 &       Type \\
\midrule
One Dose of J.\&J. Vaccine Is Ineffective Against Delta, Study Suggests &	J.\&J. Vaccine May Be Less Effective Against Delta, Study Suggests & 0.6830 & no label \\
Malawi burns thousands of Covid-19 vaccine doses&	Malawi burns thousands of expired AstraZeneca Covid-19 vaccine doses & 0.7217 & no label \\
Biden to huddle with Senate Democrats on Covid relief ahead of push for passage&	Biden urges Senate Democrats to reject poison pills that could sink relief plan ahead of push for passage & 0.3777 & no label \\
Australia to investigate two deaths for possible links to COVID-19 vaccine&	Australia says two deaths not likely to be linked to COVID-19 vaccine & 0.7236 & citation \\
Canada adds blood clot warning to AstraZeneca's COVID-19 vaccine &	Canada says AstraZeneca COVID-19 vaccine safe, but adds blood clot warning & 0.7546 & citation \\
China's Zhurong rover will land on Mars TONIGHT	& China's Zhurong rover will land on Mars 'in the next five days & 0.7234 & no label \\
Nike chief executive says firm is 'of China and for China'	&Nike boss defends firm's business in China & 0.4559 & no label \\
MAGA 2.0&	“A new bargain”: Biden’s 2024 tease bets big on nostalgia & 0.0257 & emotional \\
\midrule
                                                    At Least Eight People Died In A School Shooting In Russia &                                                                          At Least Nine People Died In A School Shooting In Russia &         0.9866 &  paraphrase \\
            India sees cases officially drop below 300,000 a day but now country threatened by killer cyclone &                                      India cases officially drop below 300,000 a day but now country threatened by killer cyclone &         0.9034 &  paraphrase \\
                                                  90\% of all adults eligible for COVID-19 vaccine by April 19 &                                                                     90\% of all U.S. adults eligible for COVID vaccine by April 19 &         0.8448 &  paraphrase \\
                                               A 19th Century Theory Explains Why Consumers Might Not Splurge &                                                                      A 19th Century Theory Explains Why Consumers May Not Splurge &         0.9857 &  paraphrase \\
                                                 The cost of living posts biggest surge since 2008, CPI shows &                                The cost of living posts biggest surge since 2008, CPI shows, as inflation spreads through economy &         0.8202 &  paraphrase \\
                                                        The Latest: UN: 38,000 Palestinians displaced in Gaza &                                                                         The Latest: Biden expresses 'support' for Gaza cease-fire &         0.4043 &  dyn update \\
                                       Dyson leak row: Don't lock ministers in ivory towers, says senior Tory &                                                                                  Starmer: PM can't distance himself from 'sleaze' &         0.2030 &  dyn update \\
                               August 5 at 2PM ET: Join Engine Media CEO and Executive Chairman Fireside Chat &                                                 August 5 at 2PM ET: Join Engine Media CEO and Executive Chairman in Fireside Chat &         0.9393 &  dyn update \\
                                             Plant-Based Food Use Rising ‘Unbelievably Fast’: Catalyst Update &                                                                    FTX Chief Sees Enduring Volatility for Crypto: Catalyst Update &         0.1229 &  dyn update \\
                                                 Futures Steady Before Payrolls; Treasuries Dip: Markets Wrap &                                                                  Stocks, Treasury Yields Rise on Robust Jobs Report: Markets Wrap &         0.3799 &  dyn update \\
                                                                               23 Amazing Jokes From Hot Fuzz &                                                      23 Jokes From "Hot Fuzz" That Humans Will Laugh At For The Next 10,000 Years &         0.4715 & elaboration \\
                                Dad’s Girlfriend Arrested After Child’s Body Found in Tote Bag at Texas Motel &                                   Dad of Boy Found Dead in Tote Bag at Texas Motel ‘Can Barely Breathe’ as Girlfriend Is Arrested &         0.5259 & elaboration \\
                                          Secrets of Prince William and Kate Middleton's big day 10 years ago &                                  Royal wedding secrets from Prince William and Kate Middleton's big day on their 10th anniversary &         0.5444 & elaboration \\
                                                 Official: Haiti President Jovenel Moïse assassinated at home &                                               Haiti President Jovenel Moïse assassinated at home; Biden calls it 'very worrisome' &         0.5179 & elaboration \\
                                 'More explosions could occur': Thousands flee as volcano erupts in Caribbean &           'More explosions could occur': La Soufriere volcano eruption sends thousands fleeing on Caribbean island of St. Vincent &         0.6160 & elaboration \\
                                           Senator Capito says Republicans plan new U.S. infrastructure offer &                                                                          U.S. Senate Republicans prepare new infrastructure offer &         0.5434 &   concision \\
                                            Caroline Jurie: Mrs World arrested over Sri Lanka pageant bust-up &                                                                                 Sri Lanka Mrs World arrested over pageant bust-up &         0.6387 &   concision \\
                              U.S. stock futures take retail sales, PPI data in stride as investors await Fed &                                                                 U.S. stocks edge lower after economic data as investors await Fed &         0.5774 &   concision \\
                      U.S. second-quarter economic growth revised slightly higher; weekly jobless claims rise &                                                                        U.S. second-quarter growth raised; corporate profits surge &         0.5540 &   concision \\
                                            Right-Wing Media Attacks ‘Weak’ Simone Biles: ‘Selfish Sociopath’ &                                                                         Right-Wing Media Launches Unhinged Attack on Simone Biles &         0.4696 &   concision \\
                                                                                   FKA twigs steps out in NYC &                                     FKA twigs steps out in NYC after claiming it was a 'relief' to speak out against Shia LaBeouf &         0.5539 &   emotional \\
                       Phoebe Dynevor Almost Quit Acting Before Her "Bridgerton" Audition With Regé-Jean Page &                                      Phoebe Dynevor Wanted To "Throw In The Towel" On Her Acting Career Right Before "Bridgerton" &         0.4885 &   emotional \\
                                                 Undercover police officers spied on Peter Hain over 25 years &                                                  Peter Hain accuses undercover police of lying over reports on apartheid campaign &         0.2465 &   emotional \\
US surpasses 100M vaccinations; Pfizer vaccine appears effective against asymptomatic cases: COVID-19 updates &                        US surpasses 100M vaccinations; IRS begins sending first round of \$1,400 relief payments: COVID-19 updates &         0.4424 &   emotional \\
                                               Suspect arrested following series of Arizona traffic shootings &                                                     Arizona gunman goes on traffic shooting rampage, leaving one dead, 12 injured &         0.2247 &   emotional \\
                                            23 Funny "Brooklyn Nine-Nine" Memes To Get You Ready For Season 8 &                                                                                                Brooklyn Nine Nine Memes And Jokes &         0.2271 &  neutralize \\
                Hundreds chanting 'Kill the Bill' protest in Bristol over controversial Police and Crime bill &                                    Protesters smash police windows and attack officers' van amid 'Kill the Bill' march in Bristol &         0.4220 &  neutralize \\
                 Prince Philip will become 25th Royal in a 200-year-old vault hidden below St George's Chapel &                               Prince Philip to be buried in 200-year-old vault below St George's Chapel but only until Queen dies &         0.6037 &  neutralize \\
                                                 Raul Castro confirms he's resigning, ending long era in Cuba &                                                                        Raul Castro resigns as Communist chief, ending era in Cuba &         0.7310 &  neutralize \\
         Nikki Grahame's life will be celebrated in a new Channel 4 documentary four months on from her death &                                                                   Nikki Grahame to be commemorated in a new Channel 4 documentary &         0.6698 &  neutralize \\
                                        Fourth stimulus check update: Your next payment could be one of these &                                                                 Fourth stimulus check? These payments are already in the pipeline &         0.4479 & foward ref. \\
                                                                       12 Movie Opinions You Might Agree With &                                                     Here Are 12 More Movie Opinions I Strongly Believe, But Do You Agree With Me? &         0.4246 & foward ref. \\
                    A park next to the White House that was closed amid protests last year partially reopens. &                                   Lafayette Park, which was closed amid protests at the White House last year, partially reopens. &         0.7430 & foward ref. \\
                                         Biden to share ‘next steps’ for COVID-19 booster program later today & People in the U.S. who were vaccinated with Moderna and Pfizer’s COVID-19 vaccines will be eligible for a third dose in September &         0.2475 & foward ref. \\
                                                   ‘How I Got In’: A Harvard/Stanford/Wharton Admit Tells All &                                                                          How I Got In: A Harvard/Stanford/Wharton Admit Tells All &         0.7685 & foward ref. \\
                                                 Watch Jeff Bezos’ ‘Blue Origin’ launch into space live today &                                                Everything you need to know as Jeff Bezos’ ‘Blue Origin’ launches into space today &         0.6179 & personalize \\
                                The "Degrassi: TNG" Cast Is Reuniting In Honor Of The Show's 20th Anniversary &                                                      The "Degrassi" Cast Is Reuniting And I Am So Excited To Relive My Teen Years &         0.4838 & personalize \\
                        Stimulus Update: States Give Out Thousands of Bonus \$1,000 Checks To School Employees &                                             Stimulus Update: States Give Out Thousands of Bonus \$1,000 Checks – Will You Get One? &         0.7416 & personalize \\
         Chrissy Teigen shares embarrassing encounter with Michael Keaton while playing game on NBC talk show &                                   Chrissy Teigen reveals she once confused Hollywood legend Michael Keaton for a champagne WAITER &         0.3173 & personalize \\
       ‘Strong perception’ that Tory party is insensitive to Muslim communities, report finds – politics live &                       Boris Johnson says he would not repeat ‘offending language’ about Muslims as prime minister – politics live &         0.3395 & personalize \\
                                    Kendall Jenner Has Some Pretty Strong Thoughts About The Kardashian Curse &                                   Kendall Jenner Talked About The Kardashian Curse And Said "The Men Need To Take Responsibility" &         0.5229 &    citation \\
                                             Howard Beckett: Labour suspends union official after Patel tweet &                                                   Howard Beckett: Patel laws 'disgusting' says union boss after Labour suspension &         0.4986 &    citation \\
                  Afghan guard killed: Firefight leaves at least one dead and others injured at Kabul airport &                  'It would be better to die under Taliban rule than face airport crush', say US embassy's 'betrayed' Afghan staff &         0.0656 &    citation \\
                                                       Police: 3 officers stable after being shot in Delaware &                                                                       Police say threat over after 3 officers wounded in Delaware &         0.6105 &    citation \\
                                           Apple beats sales expectations on iPhone, services, China strength &                                                                    Apple says chip shortage reaches iPhone, growth forecast slows &         0.2611 &    citation \\
\bottomrule
\end{tabular}

\end{table}
}

\begin{figure}[ht]
    \centering
    \includegraphics[width=0.95\textwidth]{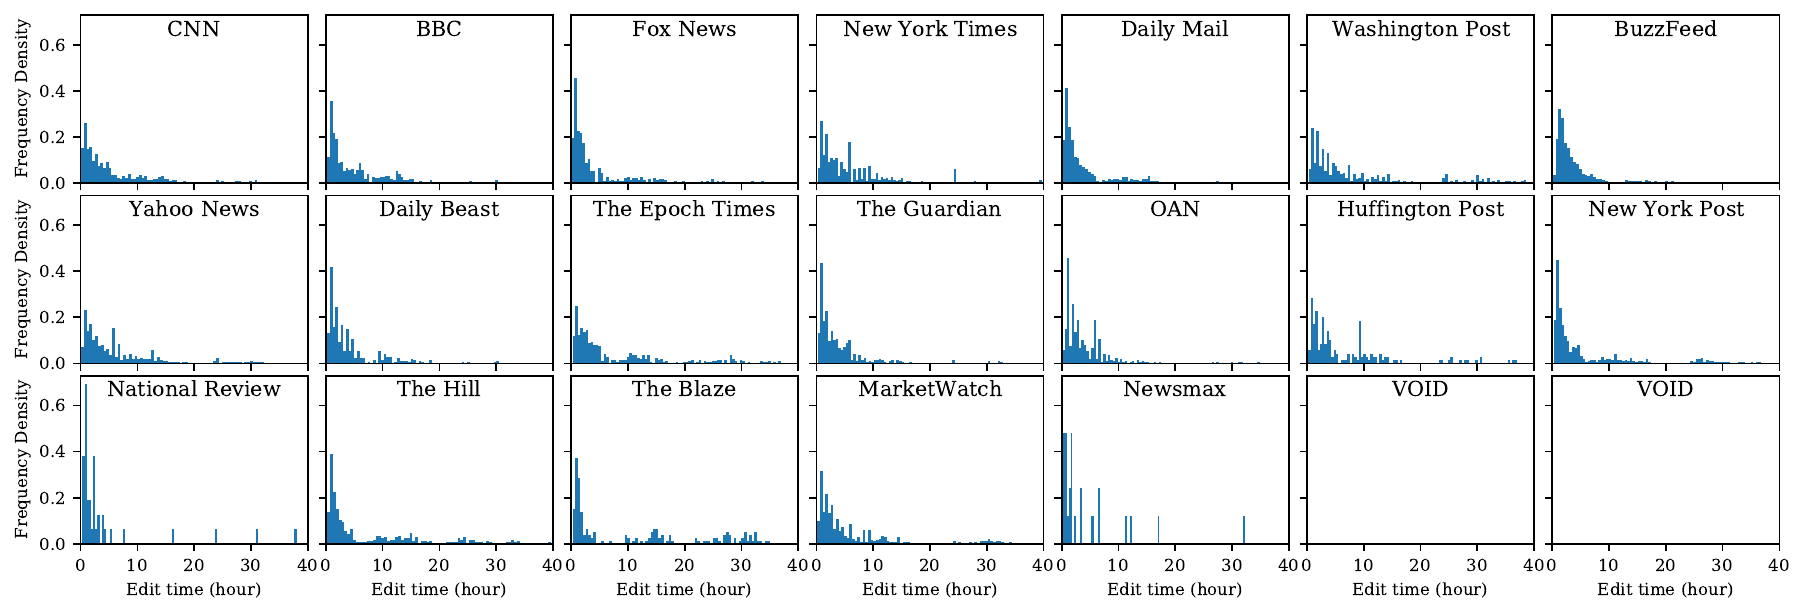}
    \caption{The post-publication edit time per news publisher. }
    \label{fig:edit-time-per-agent}
\end{figure}

\xingzhiswallow{
\begin{figure}
    \centering
    \includegraphics[height=1.0\textheight]{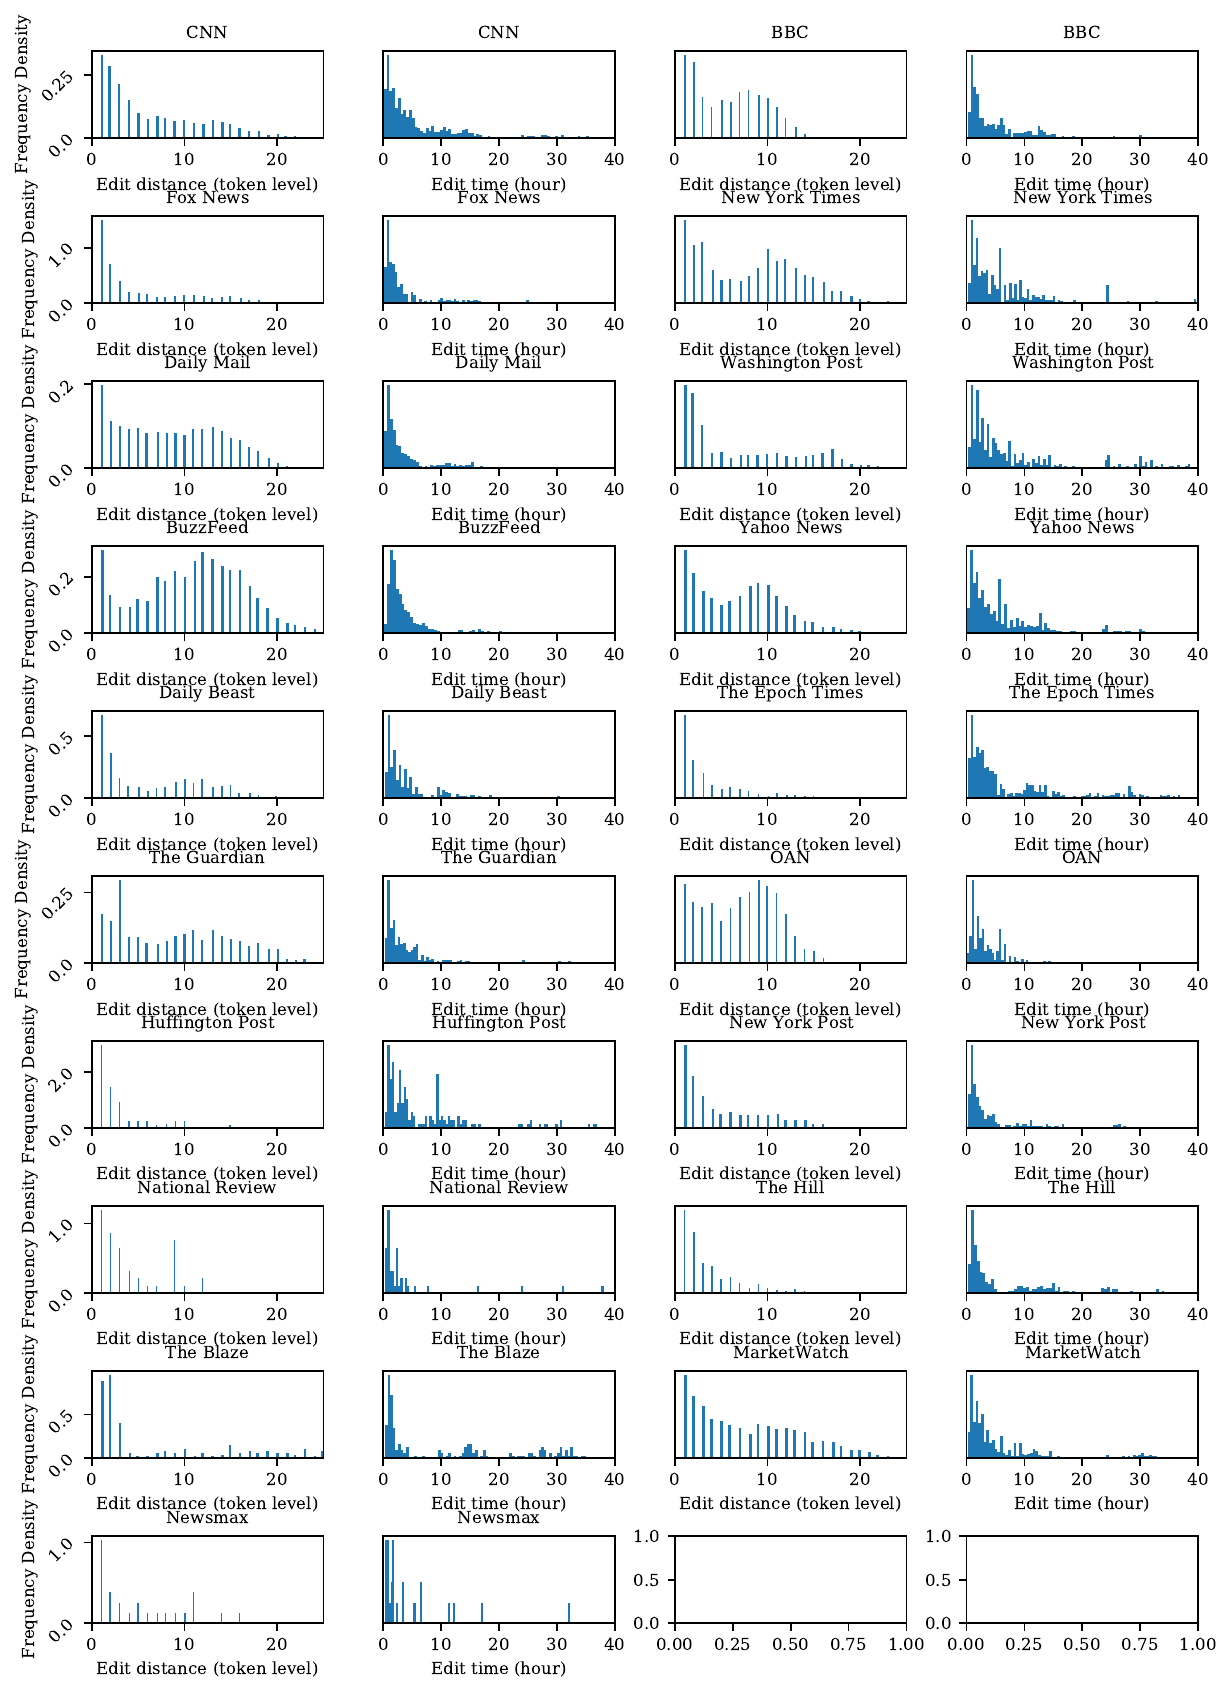}
    \caption{The edit distance and edit time per agency}
    \label{fig:edit-dis-time-per-agent}
\end{figure}

}

\xingzhiswallow{

\begin{table}[ht]
    \centering
    \tiny
    \caption{The tracked news category per agency}
    \label{tab:news_cate_agency}

\begin{tabular}{lrrrrrr}
\toprule
         Domain &  Politics &  Business &  Entertainment &  Technology &  Top Stories &  Total \\
\midrule
            BBC &      1973 &      1562 &           1495 &         824 &            0 &   5854 \\
       BuzzFeed &       330 &        92 &           3928 &         195 &            0 &   4545 \\
            CNN &      4548 &         1 &           1166 &         629 &            0 &   6344 \\
    Daily Beast &         0 &         0 &              0 &           0 &         4359 &   4359 \\
     Daily Mail &         0 &      3670 &          36312 &        1263 &        33873 &  75118 \\
       Fox News &      6307 &       108 &           4273 &         315 &            0 &  11003 \\
Huffington Post &      2909 &        57 &           1902 &           7 &            0 &   4875 \\
    MarketWatch &         0 &         0 &              0 &           0 &         7503 &   7503 \\
National Review &         0 &         0 &              0 &           0 &         3324 &   3324 \\
  New York Post &         0 &      1458 &           2018 &         514 &         9891 &  13881 \\
 New York Times &      2374 &      2983 &           3851 &         538 &            0 &   9746 \\
        Newsmax &       897 &        25 &            155 &          38 &            0 &   1115 \\
            OAN &      2922 &      3545 &            528 &        1328 &            0 &   8323 \\
      The Blaze &         0 &         0 &              0 &           0 &         4401 &   4401 \\
The Epoch Times &      3179 &      1077 &            193 &         316 &            0 &   4765 \\
   The Guardian &      3456 &       627 &           1874 &         959 &            0 &   6916 \\
       The Hill &         0 &         0 &              0 &           0 &         5676 &   5676 \\
Washington Post &      2126 &      2014 &           1458 &         478 &            0 &   6076 \\
     Yahoo News &     11074 &    183653 &              7 &       32512 &            0 & 227246 \\
\bottomrule
\end{tabular}
\end{table}

\begin{table}[ht]
    \centering
    \tiny
    \caption{The breakdown of change ratio in each news category per agency}
    \label{tab:in_changed_news_cate_ratio_agency}

\begin{tabular}{lrrrrrr}
\toprule
{} &  Politics &  Business &  Entertainment &  Technology &  Top Stories &  Total \\
Domain          &           &           &                &             &              &        \\
\midrule
BBC             &    0.3082 &    0.2855 &         0.1371 &      0.0898 &       0.0000 & 0.2277 \\
BuzzFeed        &    0.2576 &    0.0000 &         0.4812 &      0.2154 &       0.0000 & 0.4438 \\
CNN             &    0.2419 &    0.0000 &         0.1612 &      0.0000 &       0.0000 & 0.2030 \\
Daily Beast     &    0.0000 &    0.0000 &         0.0000 &      0.0000 &       0.1308 & 0.1308 \\
Daily Mail      &    0.0000 &    0.0515 &         0.0592 &      0.0451 &       0.0970 & 0.0756 \\
Fox News        &    0.0591 &    0.0926 &         0.0314 &      0.0571 &       0.0000 & 0.0486 \\
Huffington Post &    0.0399 &    0.0877 &         0.0273 &      0.1429 &       0.0000 & 0.0357 \\
MarketWatch     &    0.0000 &    0.0000 &         0.0000 &      0.0000 &       0.3453 & 0.3453 \\
National Review &    0.0000 &    0.0000 &         0.0000 &      0.0000 &       0.0126 & 0.0126 \\
New York Post   &    0.0000 &    0.0638 &         0.0852 &      0.0292 &       0.0650 & 0.0665 \\
New York Times  &    0.2784 &    0.3144 &         0.0444 &      0.1375 &       0.0000 & 0.1892 \\
Newsmax         &    0.0268 &    0.0400 &         0.0065 &      0.0000 &       0.0000 & 0.0233 \\
OAN             &    0.0404 &    0.4886 &         0.0890 &      0.2108 &       0.0000 & 0.2616 \\
The Blaze       &    0.0000 &    0.0000 &         0.0000 &      0.0000 &       0.0400 & 0.0400 \\
The Epoch Times &    0.1787 &    0.0706 &         0.0259 &      0.1203 &       0.0000 & 0.1442 \\
The Guardian    &    0.2922 &    0.3142 &         0.0326 &      0.1022 &       0.0000 & 0.1975 \\
The Hill        &    0.0000 &    0.0000 &         0.0000 &      0.0000 &       0.0592 & 0.0592 \\
Washington Post &    0.2413 &    0.1226 &         0.0501 &      0.1736 &       0.0000 & 0.1508 \\
Yahoo News      &    0.2390 &    0.0713 &         0.0000 &      0.1073 &       0.0000 & 0.0846 \\
\bottomrule
\end{tabular}
\end{table}

}

\xingzhiswallow{
\begin{table}[ht]
    \centering
    \tiny
    \caption{The breakdown of change ratio of news category per agency}
    \label{tab:across_changed_news_cate_ratio_agency}

\begin{tabular}{lrrrrrr}
\toprule
{} &  Politics &  Business &  Entertainment &  Technology &  Top Stories &  Total \\
Domain          &           &           &                &             &              &        \\
\midrule
BBC             &    0.4561 &    0.3346 &         0.1538 &      0.0555 &       0.0000 & 1.0000 \\
BuzzFeed        &    0.0421 &    0.0000 &         0.9370 &      0.0208 &       0.0000 & 1.0000 \\
CNN             &    0.8540 &    0.0000 &         0.1460 &      0.0000 &       0.0000 & 1.0000 \\
Daily Beast     &    0.0000 &    0.0000 &         0.0000 &      0.0000 &       1.0000 & 1.0000 \\
Daily Mail      &    0.0000 &    0.0333 &         0.3781 &      0.0100 &       0.5786 & 1.0000 \\
Fox News        &    0.6972 &    0.0187 &         0.2505 &      0.0336 &       0.0000 & 1.0000 \\
Huffington Post &    0.6667 &    0.0287 &         0.2989 &      0.0057 &       0.0000 & 1.0000 \\
MarketWatch     &    0.0000 &    0.0000 &         0.0000 &      0.0000 &       1.0000 & 1.0000 \\
National Review &    0.0000 &    0.0000 &         0.0000 &      0.0000 &       1.0000 & 1.0000 \\
New York Post   &    0.0000 &    0.1008 &         0.1863 &      0.0163 &       0.6966 & 1.0000 \\
New York Times  &    0.3585 &    0.5087 &         0.0927 &      0.0401 &       0.0000 & 1.0000 \\
Newsmax         &    0.9231 &    0.0385 &         0.0385 &      0.0000 &       0.0000 & 1.0000 \\
OAN             &    0.0542 &    0.7956 &         0.0216 &      0.1286 &       0.0000 & 1.0000 \\
The Blaze       &    0.0000 &    0.0000 &         0.0000 &      0.0000 &       1.0000 & 1.0000 \\
The Epoch Times &    0.8268 &    0.1106 &         0.0073 &      0.0553 &       0.0000 & 1.0000 \\
The Guardian    &    0.7394 &    0.1442 &         0.0447 &      0.0717 &       0.0000 & 1.0000 \\
The Hill        &    0.0000 &    0.0000 &         0.0000 &      0.0000 &       1.0000 & 1.0000 \\
Washington Post &    0.5600 &    0.2697 &         0.0797 &      0.0906 &       0.0000 & 1.0000 \\
Yahoo News      &    0.1377 &    0.6808 &         0.0000 &      0.1815 &       0.0000 & 1.0000 \\
\bottomrule
\end{tabular}

\end{table}

}

%\clearpage

\xingzhiswallow{
\begin{table}[ht]
\small
    \centering
    \caption{The statistics of semantic similarity (BERTScore) by agency (Ranked by the mean value). To clarify the similarity rankings from news reputation rankings, the ordered list does not reflect credibility.}
    \label{tab:bertscore_agency_fulltable}
\hspace*{-25pt}
% copy from: tab_bertscore_by_agency.tex
    \begin{tabular}{lrrrrr}
    \toprule
    Agency &   Mean &   Std. &  Median &    Tracked &  Mod.Ratio \\
    \midrule
    Huffington Post & 0.8292 & 0.1730 &  0.8966 &    4,875 &         0.0357 \\
    The Epoch Times & 0.8260 & 0.1740 &  0.8908 &    4,765 &         0.1442 \\
    The Hill        & 0.8087 & 0.1826 &  0.8644 &    5,676 &         0.0592 \\
    Fox News        & 0.7659 & 0.2310 &  0.8645 &   11,003 &         0.0486 \\
    New York Post   & 0.7305 & 0.2424 &  0.8174 &   13,881 &         0.0665 \\
    National Review & 0.7268 & 0.2660 &  0.8305 &    3,324 &         0.0126 \\
    The Blaze       & 0.7200 & 0.2758 &  0.8145 &    4,401 &         0.0400 \\
    CNN             & 0.6888 & 0.2531 &  0.7493 &    6,344 &         0.2030 \\
    Washington Post & 0.6840 & 0.2778 &  0.7916 &    6,076 &         0.1508 \\
    Newsmax         & 0.6733 & 0.2714 &  0.7319 &    1,115 &         0.0233 \\
    Daily Beast     & 0.6584 & 0.2915 &  0.7693 &    4,359 &         0.1308 \\
    MarketWatch     & 0.6551 & 0.2608 &  0.7011 &    7,503 &         0.3453 \\
    BBC             & 0.6031 & 0.2671 &  0.6260 &    5,854 &         0.2277 \\
    Yahoo News      & 0.5985 & 0.2801 &  0.6160 &  227,246 &         0.0846 \\
    Daily Mail      & 0.5936 & 0.2741 &  0.6348 &   75,118 &         0.0756 \\
    OAN             & 0.5830 & 0.2590 &  0.5910 &    8,323 &         0.2616 \\
    The Guardian    & 0.5579 & 0.2896 &  0.5826 &    6,916 &         0.1975 \\
    New York Times  & 0.5234 & 0.3283 &  0.5595 &    9,746 &         0.1892 \\
    BuzzFeed        & 0.5085 & 0.2529 &  0.4872 &    4,545 &         0.4438 \\
    \bottomrule
\end{tabular}
\end{table}

}

\xingzhiswallow{
\begin{table*}[t]
\caption{The breakdown of edit types per news agency. We highlight the top one in each column.}
\label{tab:change_category_by_agency_full_tablels}
\small
\centering
\hspace*{-30pt}
\begin{tabular}{lp{0.08\textwidth}p{0.08\textwidth}p{0.08\textwidth}p{0.08\textwidth}p{0.08\textwidth}p{0.08\textwidth}p{0.08\textwidth}p{0.08\textwidth}p{0.06\textwidth}p{0.08\textwidth}}
\toprule
Agency &  Paraphrase &  Dynamic Update &  Elaboration &  Concision &  Emotional &  Neutralize &  Forward Reference &  Personalize &  Citation &  \#Changed \\
\midrule
BBC             &      0.3196 &      0.3848 &       0.0278 &     0.0113 &     0.1043 &      0.0818 &       0.0180 &       0.0188 &    0.0540 &    1333 \\
BuzzFeed        &      0.1587 &      0.0203 &       0.0312 &     \textbf{0.1101} &     0.1026 &      \textbf{0.1894} &       \textbf{0.0709} &       \textbf{0.0699} &    0.0238 &    2017 \\
CNN             &      0.4262 &      0.0916 &       0.0404 &     0.0148 &     0.0699 &      0.0738 &       0.0171 &       0.0342 &    0.0435 &    1288 \\
Daily Beast     &      0.4754 &      0.1035 &       0.0246 &     0.0175 &     0.1123 &      0.0912 &       0.0386 &       0.0351 &    0.0298 &     570 \\
Daily Mail      &      0.2801 &      0.1158 &       0.0357 &     0.0144 &     0.0993 &      0.1218 &       0.0241 &       0.0521 &    0.0422 &    5681 \\
Fox News        &      0.6056 &      0.1925 &       0.0187 &     0.0093 &     0.0710 &      0.0617 &       0.0168 &       0.0224 &    0.0262 &     535 \\
Huffington Post &      \textbf{0.7356} &      0.0690 &       0.0000 &     0.0000 &     0.0345 &      0.0632 &       0.0000 &       0.0345 &    0.0230 &     174 \\
MarketWatch     &      0.3867 &      0.0872 &       0.0413 &     0.0178 &     0.0965 &      0.0799 &       0.0363 &       0.0154 &    0.0247 &    2591 \\
National Review &      0.5476 &      0.3810 &       0.0476 &     0.0000 &     0.0714 &      0.0476 &       0.0000 &       0.0238 &    0.0000 &      42 \\
New York Post   &      0.5211 &      0.0997 &       0.0336 &     0.0076 &     0.0715 &      0.0618 &       0.0336 &       0.0293 &    0.0141 &     923 \\
New York Times  &      0.2923 &      0.1171 &       0.0108 &     0.0108 &     0.1123 &      0.1432 &       0.0380 &       0.0184 &    0.0331 &    1844 \\
Newsmax         &      0.3846 &      0.3077 &       0.0385 &     0.0000 &     0.0000 &      0.0769 &       0.0000 &       0.0000 &    0.0385 &      26 \\
OAN             &      0.2692 &      0.0156 &       0.0280 &     0.0184 &     0.1029 &      0.0988 &       0.0032 &       0.0023 &    0.0271 &    2177 \\
The Blaze       &      0.5341 &      0.3239 &       \textbf{0.0625} &     0.0227 &     0.0682 &      0.0398 &       0.0227 &       0.0398 &    0.0455 &     176 \\
The Epoch Times &      0.6856 &      0.1659 &       0.0146 &     0.0204 &     0.0277 &      0.0422 &       0.0044 &       0.0087 &    0.0364 &     687 \\
The Guardian    &      0.2950 &      \textbf{0.4100} &       0.0271 &     0.0124 &     \textbf{0.1215} &      0.1164 &       0.0190 &       0.0190 &    \textbf{0.0688} &    1366 \\
The Hill        &      0.6637 &      0.2024 &       0.0268 &     0.0327 &     0.0208 &      0.0446 &       0.0089 &       0.0060 &    0.0179 &     336 \\
Washington Post &      0.4891 &      0.2205 &       0.0186 &     0.0109 &     0.0884 &      0.0797 &       0.0207 &       0.0437 &    0.0371 &     916 \\
Yahoo News      &      0.3256 &      0.1846 &       0.0150 &     0.0126 &     0.1047 &      0.0977 &       0.0156 &       0.0161 &    0.0340 &   19224 \\

\bottomrule

\end{tabular}
\end{table*}
}
