# Supplementary material for: Analyzing the Evolution of Graphs and Texts
Source: arXiv:2411.06295 source file (2024-11-09)
Supplement: Supplementary file 2 [file appendix_deprecate.tex]

\xingzhiswallow{
    
    \begin{table*}[htbp]
        \centering
        \small
    \hspace*{-0.00\textwidth}\begin{tabular}{ >{\raggedright\arraybackslash}p{0.1\textwidth} >{\raggedright\arraybackslash}p{0.03\textwidth} >{\raggedleft\arraybackslash}p{0.05\textwidth} >{\raggedright\arraybackslash}p{0.35\textwidth} >{\raggedright\arraybackslash}p{0.25\textwidth}}
    \toprule
     Category & Total & \%  & \makecell[l]{Examples (Before, After, \#)} & Description \\
    \midrule
     Share lemma & 120 & 13.48\% & \makecell[l]{(explosions, explosion, 3); (elections, election, 3)\\} & The change noun shares the lemma. \\
    \hline 
     Synonym & 73 & 8.20\% & \makecell[l]{(kids, children, 3); (address, speech,3)\\} & The change noun is synonym. \\
    \hline 
     Minor & 52 & 5.84\% & \makecell[l]{(uighurs, uyghurs, 2); (statutes, statues,1)} & Only one character is changed (excluding same lemma pairs ) \\
    \hline 
     Hyponymn  & 37 & 4.15\% & \makecell[l]{(cannabis, marijuana, 2); (semiconductor, chip, 2)\\(vote, election, 2); (shooter, gunman, 1)} & Become more specific\\
    \hline 
     Hypernymn & 62 & 6.97\% & \makecell[l]{(probe, inquiry, 7);(address, speech, 3)\\(crash, accident, 3); (hike, increase, 2)} & Become more general  \\
     \hline 
     Others  & 559 & 62.80\% & \makecell[l]{(dozens, scores, 5); (virus, coronavirus, 5)\\(updates, coverage, 4); (nfl, n.f.l, 3) } & All other noun changes \\
     \bottomrule
     All & 890 & 100\% & \makecell[l]{--} & All detected noun substitutions \\
     \bottomrule
    \end{tabular}
    
        \caption{Breakdown of changed nouns. One pair may belong to more than one category}
        \label{tab:noun_changes}
    \end{table*}
    
    \begin{table*}[htbp]
        \centering
        \small
    \hspace*{-0.00\textwidth}\begin{tabular}{ >{\raggedright\arraybackslash}p{0.1\textwidth} >{\raggedright\arraybackslash}p{0.03\textwidth} >{\raggedleft\arraybackslash}p{0.05\textwidth} >{\raggedright\arraybackslash}p{0.35\textwidth} >{\raggedright\arraybackslash}p{0.25\textwidth}}
    \toprule
     Category & Total & \%  & \makecell[l]{Examples (Before, After, \#)} & Description \\
    \midrule
     Share lemma & 114 & 21.76\% & \makecell[l]{(says, said, 4); (calls, called, 2)\\} & The change noun shares the lemma. \\
    \hline 
     Synonym & 57 & 10.88\% & \makecell[l]{(quits, resigns, 2); (slide, slip, 2)\\} & The change noun is synonym. \\
    \hline 
     Minor & 13 & 2.48\% & \makecell[l]{(benefitted, benefited, 1); (ties, tries,1)} & Only one character is changed (excluding same lemma pairs ) \\
    \hline 
     Hyponymn  & 56 & 10.69\% & \makecell[l]{(replaced, ousted, 2); (creates, causes, 2)\\(quits, resigns, 2); (supports, backs, 1)} & Become more specific\\
    \hline 
     Hypernymn & 45 & 8.59\% & \makecell[l]{(grows, becomes, 1);(assist, help, 1)\\(quits, departs, 1); (offers, proposes, 2)} & Become more general  \\
     \hline 
     Others  & 264 & 50.38\% & \makecell[l]{(lead, beat, 4); (ousted, fired, 2)\\(arrested, charged, 2); (sees, faces, 2) } & All other noun changes \\
     \bottomrule
     All & 524 & 100\% & \makecell[l]{--} & All detected verb substitutions \\
     \bottomrule
    \end{tabular}
        \caption{Breakdown of changed verbs. One pair may belong to more than one category}
        \label{tab:verb_changes}
    \end{table*}
}

\xingzhiswallow{
    \begin{table*}[htbp]
        \centering
        \small
        \hspace{-0.0\textwidth}
    \begin{tabular}{p{0.04\textwidth}p{0.015\textwidth}p{0.4\textwidth}p{0.4\textwidth}p{0.08\textwidth}}
    \toprule
     Diff. &  \# & Before & After & BERTScore\\
    \midrule
       1.0 &     116  & louisiana floods lead to 6 deaths & louisiana floods lead to 7 deaths &        0.99 \\
       2.0 &      45 &yankees lead astros 1-0 in game 1: live score and updates & yankees lead astros 3-0 in game 1: live score and updates &       0.96 \\
      -1.0 &      31 &ransomware attack hits 23 texas towns, authorities say & ransomware attack hits 22 texas towns, authorities say &       0.99 \\
      3.0 &      24 &super bowl 2020 live: chiefs lead the 49ers, 7-3 & super bowl 2020 live: chiefs lead the 49ers, 10-3 &       0.93 \\
      4.0 &      17 &iraq: suicide bombing kills at least 18 in baghdad & iraq: suicide bombing kills at least 22 in baghdad &       0.98 \\
      5.0 &      14 & albania earthquake kills at least 8 & albania earthquake kills at least 13 &       0.97 \\
    %   8.0 &      10 \\
    %   6.0 &       9 \\
    %   9.0 &       8 \\
      100.0 &       6 & iran-iraq earthquake kills more than 300 & iran-iraq earthquake kills more than 400 &       0.98 \\
    \bottomrule
    \end{tabular}
        \caption{Numerical difference between pre/post-edits of numbers in changed news titles: Most of them concern news dynamic updates of injuries, casualties and competition scores. \textit{BERTScore}, which is introduced in next subsection, measures the semantic similarity between the pre/post-edited titles. The high score means that numerical changes does not alter the sentence meaning.}
        \label{tab:numerical_changes}
    \end{table*}
}

\xingzhiswallow{
    \begin{table*}[H]
    \caption{The lower similarity between headlines was caused by different emphasis of the news content, except the example from BuzzFeed. }
    \label{tab:lowbert_example}
        \centering
        \small
    \begin{tabular}{p{0.1\textwidth} p{0.39\textwidth}p{0.37\textwidth}p{0.07\textwidth}}
    \toprule
    Agency &                                                Previous Title &                                               Modified Title &  BERTScore \\
    \midrule
              BBC &                People swap summer holidays for winter ones, says TUI &                Tui and EasyJet to offer holidays in amber countries &       0.075 \\
            %   BBC &                   Johnson cancels India trip amid rising Covid cases &      Coronavirus: 'Only sensible' to cancel India trip says Johnson &       0.077618 \\
            %   BBC &       Jack Dorsey tweet: Man who buys his first-ever post speaks out &       Twitter: Buyer defends paying \$2.9m for 'Mona Lisa' of tweets &       0.073927 \\
            %   BBC & Raab dismisses 'gossip' as he defends Johnson over flat revamp costs & Senior Tory says PM should resign if he has broken ministerial code &       0.086047 \\
            %   BBC &     UK economy to recover to pre-Covid levels this year, says Bailey &                     Bank of England 'not out of firepower' on Covid &       0.055215 \\
            % CNN & Engine debris rained over a mile across a Denver suburb. Now Boeing recommends suspending its 77... &                      Engine on United Airlines flight was showing signs of metal fatigue, NTSB says &       0.018372 \\
              CNN & Senior cybersecurity official warns attacks on US are growing more 'sophisticated frequent and a... &                  Four key takeaways on the US government response to the pipeline ransomware attack &       0.057 \\
            %   CNN &    'We've done worse than most any other country,' Fauci says as US marks grim Covid-19 death toll  & After a devastating milestone, Covid-19 vaccine makers pledge hundreds of millions of doses thro... &       0.010860 \\
            %   CNN &        Fears over potential fourth surge rise as White House sends warning to Covid-weary Americans &                        Biden pleads with states to slow openings as new Covid-19 viral surge builds &       0.095422 \\
            %   CNN &                        Biden's pick to lead Health and Human Services goes before Senate committees &                                 Republicans question Becerra on abortion and health care experience &       0.091858 \\
              NYT &                Fan Armies Are Harassing Gay and Trans People on TikTok &        Are Influencers Responsible for the Behavior of Their Followers? &       0.048 \\
    % New York Times &     Will the Government Be Open in a Week? Here Are the Dividing Lines &                       Five Key Questions as a Government Shutdown Looms &       0.091645 \\
    % New York Times &                 Is U.K. the New Terrorism Target? Or Was It All Along? &        At Least One London Assailant Was on Police Radar, Exposing Gaps &       0.081801 \\
    % New York Times &   Funerals and Fury in Beirut as Scale of Devastation Comes Into Focus & As French President Visits Beirut, Lebanese Ask Where Their Leaders Are &       0.028782 \\
    % New York Times & As Coronavirus Returns to Beijing, Schools Shut and Flights Are Halted &             Beijing’s Partial Lockdown a Sign of the World’s New Normal &       0.053006 \\
         The Guardian &                                 Hancock defends India travel ban delay as Covid variant cases mount &                             Hancock: most Bolton Covid patients eligible for jab but haven’t had it &       0.067 \\
         BuzzFeed & Tell Us About Yourself And We'll Reveal Which Oscar-Nominated Movie You Should Watch Next &     Everyone Has An Oscar Movie That Fits Their Personality — Here's Yours &       0.038 \\
    \bottomrule
    \end{tabular}
    \end{table*}

}

\xingzhiswallow{
    \begin{table*}[h]
    \caption{Descriptions and examples of nine categories for title changes}
    \label{table:label_taxonomy}
    \centering
    \small
    \begin{tabular}{p{0.14\textwidth}|p{0.20\textwidth}|p{0.05\textwidth}|p{0.08\textwidth}|p{0.2\textwidth}|p{0.2\textwidth}}
    \toprule
     Label & Description & \# & Fraction & Before & After \\
    \midrule
     Paraphrase & No new information added. High BERTScore-F1 & 9996 & 0.3078 & Bitcoin slides below \$40,000 after China's new crypto curbs & Bitcoin slides below \$40,000 after China's new crypto ban \\
    \hline 
     Dynamic update & Both old\&new have the keywords: “live updates, updates stream, :” & 8152 & 0.2510 & powell to testify as focus on economic pain persists: live updates & powell testifies as focus on economic pain persists: live updates \\
    \hline 
     Emotionalism & Only the new title has subjective words (from subjective dictionary, 4748 subjective words) & 3348 & 0.1031 & ballots are broken. we redesigned them. & good design is the secret to better democracy \\
    \hline 
     Neutralization & Only the old title has subjective words. & 2787 & 0.0858 & wedding industry workers are sharing wedding red flags that scream "this ends in divorce" & wedding workers are sharing wedding red flags that say "this ends in divorce" \\
    \hline 
     Forward Reference & Only the new title has the keywords: “why, when, who, which, how , ? ,...” & 1344 & 0.0413 & the biggest prize in e-sports: talent & how to make billions in e-sports \\
    \hline 
     Personalization & Only the new title has the keywords: “you, I ,we, he, she, my, your,…” & 1127 & 0.0347 & just a bunch of memes for everyone who’s hopelessly addicted to "the sims" & if you're addicted to "the sims" you'll love every one of these jokes \\
    \hline 
     Elaboration & New title added more descriptions: \ High BERTRecall Score, slightly low precision. & 918 & 0.0282 & britain releases radical islamist preacher under strict controls & britain releases anjem choudary, radical islamist preacher, under strict controls \\
    \hline 
     Citation & Only the new title has the keywords: “said, says, told, tell,…” & 906 & 0.0279 & doctors are covid’s first historians & this is not the flu’: what doctors say about their fight against coronavirus \\
    \hline 
     Concision & New title deleted descriptions: \ High BERT Precision Score, slightly low recall. & 717 & 0.0220 & air travel in the age of coronavirus: a visual diary of a flight & a visual diary of a flight  \\
    %\hline 
    % Spelling Correction & - & - & - & - & - \\
    %\hline 
    % Grammar Correction & ** headline has its own grammar rule & - & - & - & - \\
     \toprule
    \end{tabular}
    \end{table*}

}

\xingzhiswallow{

    \begin{table*}[]
    \centering
\begin{tabular}{lllr}
\toprule
 Parsed\_Domain &                                                                               s0\_pre\_token\_sentence &                                                                     s1\_pre\_token\_sentence &  bert\_score\_f1 \\
\midrule
           BBC &                                               People swap summer holidays for winter ones, says TUI &                                      Tui and EasyJet to offer holidays in amber countries &       0.075122 \\
        Daily Mail & Miley Cyrus steps out in a massive coat and mohawk as she leaves her New York hotel ahead of SNL... &   Elon Musk's controversial hosting gig will be streamed live to 100 countries on YouTube &       0.025800 \\
    New York Times &                                                                   Abolish the Federal Death Penalty &                 The Government Has Not Explained How These 13 People Were Selected to Die &       0.005893 \\
    New York Times &                                                       Putting the Burden of Organ Donation on Women &                                      My Father Needed a Liver. Did It Have to Be From Me? &       0.006725 \\
    New York Times &                            George Floyd Protests Updates: Memorials Planned as Nation Tries to Heal & Protest Updates: Ahmaud Arbery Suspect Used Racial Slur After Shooting, Investigator Says &       0.012987 \\
    New York Times &                                                       On a New York Tour, Hijabs and a Selfie Stick &                                     Tourists for a Day, Shedding Refugee Label in the Sun &       0.023581 \\
    New York Times &                                        Storm Relief Should Be Tied to Debt-Limit Bill, Mnuchin Says &                                  Harvey Aid Fight Escalates as a Weary Texas Seeks Solace &       0.047008 \\
    New York Times &                                                      Jobs Report for June: Here’s What to Watch For &                              U.S. Added 213,000 Jobs in June; Unemployment Ticks Up to 4\% &       0.059835 \\
    New York Times &                                    Police in N.Y.C. Enforcing Social Distancing Rules: Live Updates &                                                    Watch Now: Cuomo Speaks on Coronavirus &       0.061745 \\
    New York Times &                                                The Met Is Right to Reject the Sacklers’ Blood Money &                                       When Your Money Is So Tainted Museums Don’t Want It &       0.071856 \\
    New York Times &                                                               October Jobs Report: What to Look For &                                  U.S. Added 128,000 Jobs in October; Unemployment at 3.6\% &       0.073600 \\
    New York Times &                                                                Making Age Spots a Thing of the Past &                                                            Have We Aged Out of Age Spots? &       0.080818 \\
    New York Times &                                            What’s at Stake for L.G.B.T.Q. Families in This Election &                        The Most Powerful Man in the World Thinks My Family Is ‘Less Than’ &       0.083451 \\
    New York Times &                                                                          When America Bombed Itself &                      It’s Been 75 Years, and America Still Won’t Admit a Nuclear Disaster &       0.084789 \\
    New York Times &                                                                                Lebanon Is Exhausted &                             We Lebanese Thought We Could Survive Anything. We Were Wrong. &       0.090108 \\
        Yahoo News &                                                          Furlough keeps lid on soaring unemployment &                                      Drop in foreign workers in the UK less than expected &       0.034281 \\
        Yahoo News &                                            The Latest: Pfizer-BioNTech seek vaccine OK for children &                                The Latest: India sets record of 386,000 daily virus cases &       0.040589 \\
        Yahoo News &                                        Pipeline officials hope most service will be back by weekend &                              After Colonial pipeline attack, maneuvers to avert shortages &       0.064490 \\
        Yahoo News &                                     UK's Johnson launches mass testing programme as economy reopens &              Too soon to say if Britons can take summer holiday abroad, says UK's Johnson &       0.065017 \\
        Yahoo News &                                   U.S. stocks close mixed as Dow notches fifth straight record high &                                      S\&P 500, Nasdaq weighed down by spike in bond yields &       0.065980 \\
    \bottomrule
    \end{tabular}    \caption{Caption}
        \label{tab:my_label}
    \end{table*}
    
    \begin{table}[]
        \centering
    \begin{tabular}{lllr}
    \toprule
     Parsed\_Domain &                                                                  s0\_pre\_token\_sentence &                                                                             s1\_pre\_token\_sentence &  bert\_score\_f1 \\
    \midrule
          BuzzFeed &          Here Are The Eye-Opening Things An Adult Entertainer Had To Say About Her Job & We Asked An Adult Entertainer The Questions You Had About Her Job, And Here's What She Had To Say &       0.505347 \\
        Daily Mail & Katherine Schwarzenegger gushes about 'clicking very quickly' with husband Chris Pratt &                Katherine Schwarzenegger says she knew husband Chris Pratt was The One 'right away &       0.493350 \\
    New York Times &                                    Golf Takes a Do-Over and Resets Its Majors Schedule &                                             Golf Takes a Do-Over as the Masters Moves to November &       0.455645 \\
    New York Times &                        Goldman Sachs Is Drawn Into Prosecution of Vast Financial Fraud &                                                Goldman Sachs Ensnarled in Vast 1MDB Fraud Scandal &       0.468713 \\
    New York Times &                  Suspect in Bombing That Killed 21 in Colombia Belonged to Rebel Group &                             Colombia Car Bombing Suspect Belonged to Rebel Group, Government Says &       0.468725 \\
    New York Times &                  As Trump Sounds Urgent Note on Travel Ban, a Vetting Revamp Grinds On &                                  Despite Trump’s Tough Talk on Travel Ban, Few Changes to Vetting &       0.482301 \\
    New York Times &                Jersey City Shooting: ‘Man with the Nice Smile’ Killed at Kosher Market &                               Jersey City Shooting: Immigrant With ‘Big Dreams’ Was Among Victims &       0.487243 \\
    New York Times &                                             Uber’s C.E.O. Search Is Nearing a Decision &                                 Uber Chooses Expedia’s Chief as C.E.O., Ending Contentious Search &       0.489926 \\
    New York Times &                             Fiery Explosions Erupt at Dozens of Homes in Massachusetts &                                Explosions Erupt at Dozens of Homes in Andover and Lawrence, Mass. &       0.491614 \\
    New York Times &                               Women Lead Nationwide Strike in Poland Over Abortion Law &                           Polish Women Lead Strike Over Abortion Ruling Amid Threats of Crackdown &       0.500336 \\
    New York Times &                  Alabama vs. Clemson Live: Bo Scarbrough Gives Crimson Tide Early Lead &                   Alabama vs. Clemson Live: Deshaun Watson Struggles Against Crimson Tide Defense &       0.501059 \\
    New York Times &                    Full Appeals Court Agrees to Hear Request to End Michael Flynn Case &                          Appeals Court Erases Order to End Michael Flynn Case, Sets New Arguments &       0.505287 \\
    New York Times &                                     U.S. Strikes Deal to Lift Sanctions on China’s ZTE &                                 ZTE of China to Pay \$1 Billion Fine in Deal to End U.S. Sanctions &       0.509082 \\
    New York Times &                            Mars InSight Landing: Watch NASA’s Return to the Red Planet &                                         NASA’s Mars InSight Mission Lands on Red Planet’s Surface &       0.517980 \\
    New York Times &                                      Did New York City’s Population Fall? Yes. And No. &                                              Is New York City’s ‘Remarkable Growth Story’ Ending? &       0.520642 \\
    New York Times &                                 Dario Fo, Nobel-Winning Italian Playwright, Dies at 90 &                                   Dario Fo, Whose Plays Won Praise, Scorn and a Nobel, Dies at 90 &       0.521685 \\
    New York Times &                            Tens of Thousands March in Hong Kong, Defying Face Mask Ban &                                 Hong Kong Rallies Turn Violent After Thousands Defy Face Mask Ban &       0.525118 \\
    New York Times &              Passenger Plane Stolen by Employee Crashes on Island Near Seattle Airport &                        Stolen Plane Crashes After Airline Employee Takes Off From Seattle Airport &       0.526044 \\
        Yahoo News &                             The Latest: Hearing on Capitol riot wraps; little new info &                                         The Latest: Maloney seeks answers in Capitol riot hearing &       0.492205 \\
        Yahoo News &                         Stocks Steady; Nasdaq Futures Rise as Yields Dip: Markets Wrap &                                   Futures Edge Up as Yields Dip; Turkish Lira Sinks: Markets Wrap &       0.513659 \\
    \bottomrule
    \end{tabular}    \caption{Caption}
        \label{tab:my_label}
    \end{table}
    
    \begin{table*}[]
        \centering
    \begin{tabular}{lllr}
    \toprule
     Parsed\_Domain &                                                                   s0\_pre\_token\_sentence &                                                                   s1\_pre\_token\_sentence &  bert\_score\_f1 \\
    \midrule
               BBC &                              UK sends Royal Navy to patrol Jersey port amid fishing row &                 UK sends Royal Navy ships to patrol Jersey amid fishing row with France &       0.821734 \\
        Daily Mail &                               NASA's Ingenuity helicopter prepares for its first flight &            NASA's Ingenuity helicopter prepares for first flight across surface of Mars &       0.752503 \\
    New York Times &               ISIS Member Wanted in Murder in Iraq Is Arrested in Sacramento, U.S. Says &                                           ISIS Member Arrested in Sacramento, U.S. Says &       0.752347 \\
    New York Times &                                         N.F.L. Live: Anthem Protests; Cowboys Lead Rams &                                 N.F.L. Week 4: Anthem Protests; Patriots Trail Panthers &       0.755399 \\
    New York Times & Cardinal Pell’s Legacy in Australia: Catholic Church’s Bank Is Full, but Pews Are Empty &                        In Australia, Catholic Church’s Bank Is Full, but Pews Are Empty &       0.766757 \\
    New York Times &                          N.B.A. Draft Live Updates: Knicks Select R.J. Barrett at No. 3 &                        N.B.A. Draft Live Updates: Hawks Select De’Andre Hunter at No. 4 &       0.774912 \\
    New York Times &                   Florida Begins Yet Another Recount of Senate Votes, This Time by Hand &                              Florida Recounts Senate Votes Yet Again, This Time by Hand &       0.785052 \\
    New York Times &                             Trump Says ‘Good Chance’ U.S. Reaches Trade Deal With China &                         Trump Sees ‘Good Chance’ of U.S. Reaching Trade Deal With China &       0.804355 \\
    New York Times &                                               Watch: VP Debate Live Stream and Analysis &                                               Watch Live: VP Debate Stream and Analysis &       0.808450 \\
    New York Times &                                            Trump Walks Out on Democrats After 3 Minutes &                                   Trump Walks Out on Pelosi and Schumer After 3 Minutes &       0.809956 \\
    New York Times &                                       Theresa May Quiets the Critics — in Her Own Party &                               Theresa May Quiets Brexit Deal Critics — in Her Own Party &       0.813220 \\
    New York Times &              Trump Grants Clemency to Rod Blagojevich, Bernard Kerik and Michael Milken &                                  Trump Grants Clemency to Blagojevich, Milken and Kerik &       0.823367 \\
    New York Times &           Stock Markets in Asia Rise as Investors Eye Reopenings: Live Business Updates &                            Stock Markets Rise as Investors Eye Reopenings: Live Updates &       0.832658 \\
    New York Times &                                        Coronavirus Live Updates: U.S. Cases Grow to 251 &                                 Coronavirus Live Updates: U.S. Cases Pass More than 250 &       0.833882 \\
    New York Times &      Roy Horn, Illusionist Who Dazzled Audiences as Half of Siegfried \& Roy, Dies at 75 &                   Roy Horn,Who Dazzled Audiences as Half of Siegfried \& Roy, Dies at 75 &       0.847595 \\
        Yahoo News &                           Leaked Navy video appears to show U.F.O. off California coast &                                    Leaked Navy video appears to show UFO off California &       0.756646 \\
        Yahoo News &                  Why mass shootings stopped in 2020 — and why they are now roaring back &           Op-Ed: Why mass shootings stopped in 2020 — and why they are now roaring back &       0.757851 \\
        Yahoo News &                                                    Biden's border czar is stepping down &                                   Biden's border czar Roberta Jacobson is stepping down &       0.767924 \\
        Yahoo News &       Myanmar's junta says will strive for democracy after warning anti-coup protesters &     Myanmar's junta says will strive for democracy after chilling warning to protesters &       0.773524 \\
        Yahoo News &         House GOP leader opposes bill to create commission to study Jan. 6 Capitol riot & Kevin McCarthy comes out against bill to create commission to study Jan. 6 Capitol riot &       0.784304 \\
    \bottomrule
    \end{tabular}    \caption{Caption}
        \label{tab:my_label}
    \end{table*}
    
    \begin{table*}[]
        \centering
    \begin{tabular}{lllr}
    \toprule
     Parsed\_Domain &                                                                               s0\_pre\_token\_sentence &                                                                               s1\_pre\_token\_sentence &  bert\_score\_f1 \\
    \midrule
          BuzzFeed &      Emma Stone Talked About How She Transformed Into Cruella De Vil And I Couldn't Be More Excited &     Emma Stone Talked About How She Transformed Into Cruella De Vil, And I Couldn't Be More Excited &       0.981295 \\
       MarketWatch & After a disagreement, my aunt took over as my grandmother’s power of attorney and executor of my... & After a disagreement, my aunt took over as my grandmother’s power of attorney and executor of my... &       0.986362 \\
    New York Times &                                Samsung Halts Production of Galaxy Note 7 as Battery Problems Linger &                                   Samsung Halts Galaxy Note 7 Production as Battery Problems Linger &       0.950506 \\
    New York Times &                              Stephen Miller, Trump’s Defender-in-Chief, Is Late Night’s New Nemesis &                              Stephen Miller, Trump’s Defender in Chief, Is Late Night’s New Nemesis &       0.954387 \\
    New York Times &                                    Inside the Elementary School Where Addiction Sets the Curriculum &                               Inside the Elementary School Where Drug Addiction Sets the Curriculum &       0.955816 \\
    New York Times &                                     U.S. Chamber of Commerce Names Its First New Leader in 24 Years &                                         U.S. Chamber of Commerce Names First New Leader in 24 Years &       0.957949 \\
    New York Times &                                    Migrant Children Moved Back to Troubled Border Facility in Texas &                                       Migrant Children Moved Back to Troubled Texas Border Facility &       0.960026 \\
    New York Times &                                ‘We Ran Out of Space’: Bodies Pile Up as N.Y. Struggles to Bury Dead &                            ‘We Ran Out of Space’: Bodies Pile Up as N.Y. Struggles to Bury Its Dead &       0.963992 \\
    New York Times &                    Detentions at southwestern border rose in April to highest in at least 20 years. &              Detentions at southwestern border rose in April to highest level in at least 20 years. &       0.967148 \\
    New York Times & Amy Dorris, a former model, accuses Donald Trump of sexually assaulting her at the U.S. Open in ... &      Amy Dorris, a former model, accuses Trump of sexually assaulting her at the U.S. Open in 1997. &       0.967499 \\
    New York Times &                                       Gary Cohn Said He Will Resign as Trump’s Top Economic Adviser &                                       Gary Cohn Says He Will Resign as Trump’s Top Economic Adviser &       0.976145 \\
    New York Times &                                                Soldier Kills at Least 17 in Thailand Shooting Spree &                                                Soldier Kills at Least 20 in Thailand Shooting Spree &       0.982447 \\
    New York Times &                 Coronavirus Live Updates: Trump’s Europe Travel Ban Is Met With Confusion and Anger &                 Coronavirus Live Updates: Trump’s Europe Travel Ban Is Met With Anger and Confusion &       0.984282 \\
          The Hill &                                  CEO of \$2 billion company pushed out for taking LSD before meeting &                                         CEO of \$2B company pushed out for taking LSD before meeting &       0.971835 \\
        Yahoo News &  FintechOS nabs \$61.5M for a low-code approach to modernizing legacy banking and insurance services &    FintechOS nabs \$60M for a low-code approach to modernizing legacy banking and insurance services &       0.956645 \\
        Yahoo News &                                   U.S. sanctions two Chinese officials over alleged Xinjiang abuses &                              U.S. sanctions two more Chinese officials over alleged Xinjiang abuses &       0.957248 \\
        Yahoo News & Rick Scott says he gave Trump 'Champion for Freedom' award after the Capitol insurrection becaus... & Rick Scott says he gave Trump a 'Champion for Freedom' award after the Capitol insurrection beca... &       0.959179 \\
        Yahoo News &                                            US, China spar in first face-to-face meeting under Biden &                                           US and China spar in 1st face-to-face meeting under Biden &       0.963872 \\
        Yahoo News &                     U.S. backs distance of three feet between students, which may help schools open &                         U.S. backs distance of 3 feet between students, which may help schools open &       0.991934 \\
        Yahoo News &                                       Suspected migrant boat breaks up off San Diego, killing three &                                        Suspected migrant boat breaks up off San Diego, killing four &       0.992417 \\
    \bottomrule
    \end{tabular}    \caption{Caption}
        \label{tab:my_label}
    \end{table*}
    
    \begin{table*}[]
        \centering
    \begin{tabular}{lllr}
    \toprule
     Parsed\_Domain &                                                                           s0\_pre\_token\_sentence &                                                                            s1\_pre\_token\_sentence &  bert\_score\_f1 \\
    \midrule
          BuzzFeed &                                               19 Celeb BFFs People Are Absolutely Obsessed With &                               19 Famous Friends Who Just Support And Love Each Other So Adorably &       0.290146 \\
        Daily Mail &            Joanna Lumley won't watch The Crown because viewers don't know it's 'mostly made up' &                    Joanna Lumley tells podcast Netflix series The Crown and Megxit are 'ghastly' &       0.258068 \\
        Daily Mail & Zulu war of succession: Hundreds of warriors escort Queen Mantfombi's body through Johannesburg &        Claims Zulu Queen Mantfombi was poisoned by rivals after King Goodwill Zwelithini's death &       0.314230 \\
    New York Times &                                   Confronting Iran at Sea Is an Iranian-American Navy Commander &                            He Fled Iran as a Child. Now He’s Commanding a U.S. Aircraft Carrier. &       0.257457 \\
    New York Times &                            North Korea Cuts Diplomatic Ties with Malaysia Over U.S. Extradition &                           For the First Time, a North Korean Is Set to Be Extradited to the U.S. &       0.267519 \\
    New York Times &                     Fake News and Bots May Be Worrisome, but Their Political Power Is Overblown &                                        Fake News Sways Elections, Right? Sorry, That’s Fake News &       0.273021 \\
    New York Times &                             Trump Condemns Violence in Charlottesville, Saying ‘Racism Is Evil’ &                                                    Trump Condemns Racists but Creates New Uproar &       0.275176 \\
    New York Times &                           In Denying Minimizing Threat of Virus, Trump Again Downplays Pandemic &                         Trump, in Philadelphia, Says He ‘Up-Played’ the Virus, Then Downplays It &       0.275760 \\
    New York Times &                                                                          Your Thursday Briefing &                                  Climate, Reparations, Women’s World Cup: Your Thursday Briefing &       0.286259 \\
    New York Times &                    Changing Course, Trump Accuses Saudis of ‘Deception’ in Killing of Khashoggi &                  Bipartisan Chorus Calls for Punishing Saudis; Trump Accuses Them of ‘Deception’ &       0.303229 \\
    New York Times &                    Covid-19 Live Updates: Drugmaker Has Begun Final Tests of a One-Shot Vaccine & Covid-19 Live Updates: Top U.S. Health Officials Try to Defend Their Integrity Before the Senate &       0.303603 \\
    New York Times &                                                                            Your Monday Briefing &                                                    Hong Kong, India, China: Your Monday Briefing &       0.307791 \\
    New York Times &                                             F.B.I. Reviewing New Emails in Hillary Clinton Case &                         New Emails in Clinton Case Came From Anthony Weiner’s Electronic Devices &       0.323426 \\
    New York Times &                    Trump’s Abrupt ‘Yes’ to North Korea: The 45 Minutes That Could Alter History &                                     With Snap ‘Yes’ in Oval Office, Trump Gambles on North Korea &       0.327772 \\
    New York Times &                           Report Shows Widespread Russian Interference in U.K. Political System &                          ‘No One’ Protected British Democracy From Russia, U.K. Report Concludes &       0.331616 \\
    New York Times &                                Woman Says She Was Bullied, Bound and Gagged at Work in Scotland &                        Bound and Gagged With Duct Tape at Work, She Takes On Scottish Government &       0.333774 \\
    New York Times &                                   For Trump, Threats but Few Options in Confronting North Korea &                               What Can Trump Do About North Korea? His Options Are Few and Risky &       0.336886 \\
        Yahoo News &                   India Covid-19 second wave: Shortage of oxygen, beds and even cremation slots &                                    Covid-19 in India: Why second coronavirus wave is devastating &       0.260244 \\
        Yahoo News &                                      Air havoc as passengers return ahead of summer travel boom &                                      Airlines add layovers, change travel dates as fliers return &       0.317084 \\
        Yahoo News &                      Administrators lay off 440 workers at collapsed lender Greensill: Guardian &                                                  Greensill administrators lay off some 440 staff &       0.339471 \\
        \end{tabular}
    \bottomrule
        \caption{Caption}
        \label{tab:my_label}
    \end{table*}
}
