# Supplementary material for: Analyzing the Evolution of Graphs and Texts
Source: arXiv:2411.06295 source file (2024-11-09)
Supplement: Supplementary file 3 [file chapter_appendix.tex]

\subsection{Details of Hashtag and Occupation in Ethnicity Groups}
Table \ref{tab:hashtag_category} shows the hashtags representing interested topics. Table \ref{tab:ethnicity_over_under_occ_long} shows over/under-represented occupations in each ethnicity group. 

\begin{table}[ht]
\centering
\small
\caption{Categorized hashtags. We only select hashtags that are popular and directly related to a specific topic.}
\label{tab:hashtag_category}

\begin{tabular}{p{0.20\textwidth}|p{0.45\textwidth}|p{0.1\textwidth}}
%\begin{tabular}{>{\centering\arraybackslash}m{0.13\textwidth}|p{0.2\textwidth}|p{0.1\textwidth}}
\toprule
 Category & Examples & \#Hashtags \\
\midrule 
 sports & \#nba, \#nhl & 67 \\
\hline 
 politics & \#trump, \#maga & 47  \\
\hline 
 entertainment & \#grammys, \#film, \#comedy & 25 \\
\hline 
 literature & \#bookboost, \#mustread & 16 \\
\hline 
 tech & \#tech, \#bigdata, \#science, \#ai  & 14 \\
\hline 
 business & \#digitalmarketing, \#entrepreneur & 12 \\
\hline 
 music &  \#hiphop, \#newmusic, \#music & 6 \\
 \bottomrule
\end{tabular}
\end{table}

\subsection{Model Configs.}
Table \ref{tab:model_cofig} lists the hyper-parameters for the models. We use grid search or hidden dim $\in [32,64,...,512]$,  learning rate $\in [1e-1, 1e-3,1e-5]$, freeze layer $\in [0, 5, 10, 12]$ to determine the best combinations as the model configurations. 
\begin{table}[ht]
    \centering
    \small
    \caption{Model Configuration }
    \label{tab:model_cofig}
    \hspace{0.03\textwidth}\begin{tabular}{p{0.19\linewidth}|p{0.9\linewidth}}
        \toprule
        Model & Config. Descriptions \\
        \midrule
        BiLSTM &  2 layers of Bi-directional LSTM with hidden dim = 128, 2 linear layers with Sigmoid as activation function. learning rate = 1e-03, max epoch = 10\\
        \hline
        RoBerta-CLS & Pre-trained RoBerta, 2 linear layers with ReLu activation function, linear hidden dim = 256, freeze layer = 0, learning rate = 1e-5, max epoch = 10\\
        \hline
        BERTweet & Pre-trained BERTweet, linear hidden dim = 256, freeze layer = 0, learning rate = 1e-5, max epoch = 10\\
        \bottomrule
    \end{tabular}
\end{table}

\begin{table}[ht]
% \begin{sidewaystable}[ht]
    \tiny
    \centering
    \caption{Top over/under-represented occupations in each ethnicity group (Occupation mentioned time $<$ 60): The column \textit{Ratio} measures how many time the calculated value exceeds the expected balanced value.  We break ties by sorting occupation mentioned times in descending order. }
    \label{tab:ethnicity_over_under_occ_long}
    \begin{tabular}{p{0.20\textwidth}p{0.03\textwidth}p{0.2\textwidth}p{0.03\textwidth}p{0.2\textwidth}p{0.03\textwidth}p{0.2\textwidth}p{0.03\textwidth}}
    \toprule
                           White &     Ratio &                    Asian &     Ratio &                      Hispanic &     Ratio &                          African-American &     Ratio \\
    \midrule
    \multicolumn{8}{c}{Over-represented} \\
    \midrule
              golf professional &                   2.12 &                research scholar &                   6.60 &             industrial engineer &                      3.48 &               performing artist &                  1.82 \\
                     golf coach &                   2.10 &            chartered accountant &                   5.76 &               volleyball player &                      2.30 &                    forex trader &                  1.81 \\
                 pitching coach &                   2.09 &               political analyst &                   4.08 &          industrial engineering &                      2.18 &            motivational speaker &                  1.79 \\
      assistant superintendent &                   2.07 &                   social worker &                   3.82 &                   soccer player &                      2.14 &               radio personality &                  1.75 \\
         social studies teacher &                   2.07 &            electronics engineer &                   3.49 &               medical assistant &                      1.74 &                    music artist &                  1.73 \\
              athletic director &                   2.06 &                     it engineer &                   3.43 &            full stack developer &                      1.67 &                recording artist &                  1.71 \\
                     pe teacher &                   2.06 &               android developer &                   3.38 &               computer engineer &                      1.66 &                      rap artist &                  1.71 \\
                 baseball coach &                   2.05 &                 it professional &                   3.21 &                flight attendant &                      1.64 &                     song writer &                  1.70 \\
      assistant baseball coach &                   2.04 &                  prime minister &                   3.18 &                systems engineer &                      1.63 &                      event host &                  1.67 \\
                sports director &                   2.04 &             electrical engineer &                   2.94 &                  medical doctor &                      1.57 &                 college athlete &                  1.67 \\
                 softball coach &                   2.03 &             mechanical engineer &                   2.92 &                     mma fighter &                      1.54 &                   event planner &                  1.65 \\
              volleyball coach &                   2.02 &                  content writer &                   2.81 &          environmental engineer &                      1.51 &               basketball player &                  1.61 \\
                  hockey player &                   2.01 &                       secretary &                   2.78 &               community manager &                      1.50 &                  sports analyst &                  1.61 \\
     director of comm. &                   2.00 &                   growth hacker &                   2.78 &                fashion designer &                      1.49 &                 fashion stylist &                  1.60 \\
              director of sales &                   2.00 &                  civil engineer &                   2.76 &                       networker &                      1.47 &                  hip hop artist &                  1.58 \\
    \midrule
    \multicolumn{8}{c}{Under-represented}\\
    \midrule
               research scholar &                   0.84 &                  softball coach &                   0.17 &               golf professional &                      0.25 &                research scholar &                  0.74 \\
           chartered accountant &                   0.98 &        assistant football coach &                   0.18 &                  support worker &                      0.29 &             industrial engineer &                  0.76 \\
            industrial engineer &                   1.07 &        asst. baseball coach &                   0.18 &      asst. basketball coach &                      0.30 &              software architect &                  0.77 \\
          electronics engineer &                   1.12 &                  baseball coach &                   0.19 &          men's basketball coach &                      0.31 &             assistant professor &                  0.81 \\
              android developer &                   1.17 &               athletic director &                   0.20 &                      golf coach &                      0.33 &             postdoctoral fellow &                  0.83 \\
              political analyst &                   1.17 &                volleyball coach &                   0.21 &             development officer &                      0.33 &                 senior director &                  0.83 \\
                    it engineer &                   1.27 &      asst. basketball coach &                   0.21 &                 primary teacher &                      0.34 &        assistant superintendent &                  0.83 \\
                 medical doctor &                   1.29 &           offensive coordinator &                   0.22 &               athletic director &                      0.36 &                   ios developer &                  0.83 \\
              computer engineer &                   1.29 &        assistant superintendent &                   0.22 &          recruitment consultant &                      0.37 &                  pitching coach &                  0.84 \\
                  social worker &                   1.30 &                      golf coach &                   0.23 &                 chief executive &                      0.37 &                    sr. director &                  0.84 \\
                     dominatrix &                   1.31 &                  pitching coach &                   0.23 &        assistant football coach &                      0.38 &             associate professor &                  0.85 \\
                 civil engineer &                   1.32 &                     track coach &                   0.23 &          primary school teacher &                      0.38 &        senior software engineer &                  0.85 \\
          full stack developer &                   1.32 &          recruiting coordinator &                   0.23 &                        tar heel &                      0.39 &             engineering manager &                  0.85 \\
            electrical engineer &                   1.34 &               golf professional &                   0.23 &                 radio presenter &                      0.39 &                systems engineer &                  0.86 \\
              volleyball player &                   1.34 &             assistant principal &                   0.24 &                    estate agent &                      0.40 &           senior vice president &                  0.87 \\
    \bottomrule
    \end{tabular}
\end{table}
